# Supplementary material for: Simplifying Node Classification on Heterophilous Graphs with Compatible Label Propagation
Source: arXiv:2205.09389 source file (2022-11-30)
Supplement: Supplementary file 2 [file appendix_syndata_results.tex]

% \begin{table*}
% \caption{Node classification results of Syn-1 dataset. 
% % \textsuperscript{\dag} means utilise spectral features.
% }
% % \vspace{-3mm}
% \label{table:NC_experimental_results_syn_self_005}
% % \small
% \centering
% \resizebox{.7\textwidth}{!}{
% \begin{tabular}{l ccccccccccc}
% \hline
% $h$     & 0.0 & 0.1 & 0.2 & 0.3 & 0.4 & 0.5 & 0.6 & 0.7 & 0.8 & 0.9 & 1.0\\
%         & \multicolumn{11}{c}{\textbf{Train ratio $5\%$}}  \\
% MLP & 44.53${\scriptstyle\pm0.54}$ & 44.08${\scriptstyle\pm0.69}$ & 44.44${\scriptstyle\pm0.75}$ & 44.15${\scriptstyle\pm0.57}$ & 45.85${\scriptstyle\pm0.62}$ & 44.84${\scriptstyle\pm0.71}$ & 44.38${\scriptstyle\pm0.51}$ & 45.41${\scriptstyle\pm0.85}$ & 43.76${\scriptstyle\pm0.75}$ & 43.84${\scriptstyle\pm1.0}$ & 44.5${\scriptstyle\pm0.57}$  \\
% GCN & 22.44${\scriptstyle\pm0.45}$ & 24.95${\scriptstyle\pm0.42}$ & 28.63${\scriptstyle\pm0.48}$ & 33.52${\scriptstyle\pm0.45}$ & 41.73${\scriptstyle\pm0.67}$ & 51.66${\scriptstyle\pm1.52}$ & 63.4${\scriptstyle\pm0.78}$ & 74.22${\scriptstyle\pm0.74}$ & 82.5${\scriptstyle\pm0.89}$ & 90.2${\scriptstyle\pm0.3}$ & 95.69${\scriptstyle\pm0.2}$  \\
% GAT & 23.58${\scriptstyle\pm0.88}$ & 23.96${\scriptstyle\pm1.56}$ & 27.84${\scriptstyle\pm1.1}$ & 34.09${\scriptstyle\pm0.83}$ & 42.68${\scriptstyle\pm1.28}$ & 52.65${\scriptstyle\pm1.38}$ & 61.81${\scriptstyle\pm1.32}$ & 72.82${\scriptstyle\pm0.77}$ & 81.65${\scriptstyle\pm0.87}$ & 89.85${\scriptstyle\pm0.59}$ & 96.73${\scriptstyle\pm0.36}$  \\
% GCN2 & 38.08${\scriptstyle\pm2.99}$ & 38.31${\scriptstyle\pm2.99}$ & 39.11${\scriptstyle\pm1.84}$ & 41.97${\scriptstyle\pm1.33}$ & 47.2${\scriptstyle\pm2.06}$ & 52.1${\scriptstyle\pm1.74}$ & 59.64${\scriptstyle\pm1.32}$ & 68.16${\scriptstyle\pm1.29}$ & 79.58${\scriptstyle\pm0.78}$ & 91.89${\scriptstyle\pm0.22}$ & 99.39${\scriptstyle\pm0.17}$  \\
% SuperGAT & 17.65${\scriptstyle\pm1.58}$ & 19.02${\scriptstyle\pm1.67}$ & 20.9${\scriptstyle\pm1.84}$ & 24.02${\scriptstyle\pm2.37}$ & 27.04${\scriptstyle\pm2.28}$ & 30.9${\scriptstyle\pm2.77}$ & 34.0${\scriptstyle\pm3.36}$ & 42.7${\scriptstyle\pm3.12}$ & 45.89${\scriptstyle\pm4.49}$ & 49.94${\scriptstyle\pm5.31}$ & 59.19${\scriptstyle\pm4.72}$  \\
% GPRGNN & 43.32${\scriptstyle\pm1.05}$ & 42.86${\scriptstyle\pm1.16}$ & 43.71${\scriptstyle\pm0.88}$ & 44.12${\scriptstyle\pm1.59}$ & 46.42${\scriptstyle\pm2.26}$ & 51.08${\scriptstyle\pm2.56}$ & 58.42${\scriptstyle\pm2.07}$ & 71.42${\scriptstyle\pm2.72}$ & 83.66${\scriptstyle\pm1.37}$ & 93.95${\scriptstyle\pm0.73}$ & 99.32${\scriptstyle\pm0.11}$  \\
% FAGCN & 45.14${\scriptstyle\pm0.47}$ & 44.49${\scriptstyle\pm0.58}$ & 45.4${\scriptstyle\pm0.6}$ & 45.64${\scriptstyle\pm1.01}$ & 48.79${\scriptstyle\pm1.62}$ & 51.87${\scriptstyle\pm2.08}$ & 57.02${\scriptstyle\pm3.13}$ & 63.11${\scriptstyle\pm4.46}$ & 72.02${\scriptstyle\pm3.83}$ & 80.39${\scriptstyle\pm3.42}$ & 86.71${\scriptstyle\pm2.91}$  \\
% H2GCN & 41.5${\scriptstyle\pm1.17}$ & 40.07${\scriptstyle\pm0.86}$ & 40.92${\scriptstyle\pm1.04}$ & 44.59${\scriptstyle\pm1.17}$ & 51.67${\scriptstyle\pm1.3}$ & 61.25${\scriptstyle\pm1.21}$ & 71.59${\scriptstyle\pm1.24}$ & 82.42${\scriptstyle\pm1.11}$ & 89.23${\scriptstyle\pm0.88}$ & 95.29${\scriptstyle\pm0.33}$ & 98.99${\scriptstyle\pm0.13}$  \\
% CPGNN & 19.28${\scriptstyle\pm1.77}$ & 20.15${\scriptstyle\pm1.35}$ & 20.0${\scriptstyle\pm1.37}$ & 18.15${\scriptstyle\pm2.39}$ & 20.39${\scriptstyle\pm1.41}$ & 20.45${\scriptstyle\pm1.67}$ & 19.8${\scriptstyle\pm1.33}$ & 20.45${\scriptstyle\pm1.61}$ & 19.49${\scriptstyle\pm1.17}$ & 19.44${\scriptstyle\pm1.29}$ & 20.33${\scriptstyle\pm1.34}$  \\
% LP & 9.5${\scriptstyle\pm0.66}$ & 10.27${\scriptstyle\pm0.22}$ & 12.86${\scriptstyle\pm0.39}$ & 16.98${\scriptstyle\pm0.25}$ & 23.38${\scriptstyle\pm0.66}$ & 32.32${\scriptstyle\pm0.83}$ & 46.25${\scriptstyle\pm0.7}$ & 65.99${\scriptstyle\pm1.03}$ & 82.54${\scriptstyle\pm0.74}$ & 94.41${\scriptstyle\pm0.28}$ & 99.37${\scriptstyle\pm0.03}$  \\
% C\&S & 39.9${\scriptstyle\pm3.05}$ & 40.06${\scriptstyle\pm2.67}$ & 41.43${\scriptstyle\pm2.16}$ & 42.58${\scriptstyle\pm1.18}$ & 47.6${\scriptstyle\pm1.62}$ & 55.2${\scriptstyle\pm1.86}$ & 66.9${\scriptstyle\pm2.04}$ & 84.52${\scriptstyle\pm1.17}$ & 93.62${\scriptstyle\pm0.44}$ & 97.94${\scriptstyle\pm0.24}$ & 99.54${\scriptstyle\pm0.09}$  \\
% CLP & 47.94${\scriptstyle\pm0.57}$ & 44.38${\scriptstyle\pm0.61}$ & 46.51${\scriptstyle\pm0.73}$ & 49.14${\scriptstyle\pm0.85}$ & 56.52${\scriptstyle\pm1.94}$ & 66.08${\scriptstyle\pm1.82}$ & 76.28${\scriptstyle\pm1.82}$ & 84.97${\scriptstyle\pm1.63}$ & 90.98${\scriptstyle\pm1.13}$ & 95.88${\scriptstyle\pm0.59}$ & 99.35${\scriptstyle\pm0.05}$  \\
% % \rowcolor{gray!30}
% % CLP\textsuperscript{\dag} & 47.81${\scriptstyle\pm0.38}$ & 44.91${\scriptstyle\pm0.36}$ & 46.57${\scriptstyle\pm0.8}$ & 51.82${\scriptstyle\pm1.37}$ & 56.56${\scriptstyle\pm2.27}$ & 65.15${\scriptstyle\pm2.96}$ & 75.68${\scriptstyle\pm1.29}$ & 86.95${\scriptstyle\pm0.63}$ & 92.48${\scriptstyle\pm0.67}$ & 97.43${\scriptstyle\pm0.29}$ & 99.59${\scriptstyle\pm0.02}$  \\
%         & \multicolumn{11}{c}{\textbf{Train ratio $10\%$}}  \\
% MLP & 44.94${\scriptstyle\pm0.5}$ & 44.78${\scriptstyle\pm0.37}$ & 45.18${\scriptstyle\pm0.47}$ & 44.68${\scriptstyle\pm0.53}$ & 45.99${\scriptstyle\pm0.42}$ & 45.02${\scriptstyle\pm0.75}$ & 44.71${\scriptstyle\pm0.48}$ & 45.71${\scriptstyle\pm0.48}$ & 44.33${\scriptstyle\pm0.68}$ & 44.24${\scriptstyle\pm0.56}$ & 44.95${\scriptstyle\pm0.54}$  \\
% GCN & 22.99${\scriptstyle\pm0.42}$ & 25.54${\scriptstyle\pm0.43}$ & 28.95${\scriptstyle\pm0.65}$ & 33.87${\scriptstyle\pm0.34}$ & 43.17${\scriptstyle\pm0.91}$ & 53.92${\scriptstyle\pm0.68}$ & 64.46${\scriptstyle\pm0.72}$ & 74.94${\scriptstyle\pm0.84}$ & 83.91${\scriptstyle\pm0.47}$ & 90.4${\scriptstyle\pm0.31}$ & 95.91${\scriptstyle\pm0.19}$  \\
% GAT & 26.09${\scriptstyle\pm1.22}$ & 25.38${\scriptstyle\pm1.31}$ & 30.76${\scriptstyle\pm1.27}$ & 35.05${\scriptstyle\pm1.0}$ & 45.02${\scriptstyle\pm1.03}$ & 54.07${\scriptstyle\pm1.21}$ & 64.08${\scriptstyle\pm0.73}$ & 74.28${\scriptstyle\pm0.51}$ & 82.54${\scriptstyle\pm0.43}$ & 90.38${\scriptstyle\pm0.46}$ & 97.12${\scriptstyle\pm0.33}$  \\
% GCN2 & 42.3${\scriptstyle\pm1.08}$ & 42.49${\scriptstyle\pm1.67}$ & 42.2${\scriptstyle\pm1.13}$ & 43.18${\scriptstyle\pm0.85}$ & 49.26${\scriptstyle\pm1.35}$ & 53.94${\scriptstyle\pm0.77}$ & 60.92${\scriptstyle\pm0.96}$ & 69.86${\scriptstyle\pm0.85}$ & 80.28${\scriptstyle\pm0.74}$ & 92.32${\scriptstyle\pm0.37}$ & 99.53${\scriptstyle\pm0.1}$  \\
% SuperGAT & 17.33${\scriptstyle\pm2.02}$ & 18.92${\scriptstyle\pm1.49}$ & 21.48${\scriptstyle\pm2.36}$ & 25.19${\scriptstyle\pm1.73}$ & 27.44${\scriptstyle\pm1.93}$ & 32.1${\scriptstyle\pm2.49}$ & 37.48${\scriptstyle\pm4.15}$ & 44.07${\scriptstyle\pm3.76}$ & 48.16${\scriptstyle\pm4.43}$ & 52.6${\scriptstyle\pm6.83}$ & 62.38${\scriptstyle\pm9.21}$  \\
% GPRGNN & 44.44${\scriptstyle\pm0.79}$ & 43.84${\scriptstyle\pm0.49}$ & 45.1${\scriptstyle\pm0.8}$ & 45.38${\scriptstyle\pm0.73}$ & 49.7${\scriptstyle\pm1.55}$ & 53.99${\scriptstyle\pm1.61}$ & 61.65${\scriptstyle\pm1.46}$ & 74.02${\scriptstyle\pm2.12}$ & 85.18${\scriptstyle\pm1.13}$ & 94.52${\scriptstyle\pm0.79}$ & 99.41${\scriptstyle\pm0.11}$  \\
% FAGCN & 45.4${\scriptstyle\pm0.46}$ & 44.65${\scriptstyle\pm0.77}$ & 45.56${\scriptstyle\pm0.5}$ & 46.46${\scriptstyle\pm0.77}$ & 50.49${\scriptstyle\pm1.04}$ & 53.0${\scriptstyle\pm2.3}$ & 57.99${\scriptstyle\pm2.97}$ & 65.55${\scriptstyle\pm3.49}$ & 72.13${\scriptstyle\pm4.84}$ & 81.49${\scriptstyle\pm3.95}$ & 88.51${\scriptstyle\pm2.54}$  \\
% H2GCN & 43.42${\scriptstyle\pm0.72}$ & 42.06${\scriptstyle\pm0.67}$ & 43.38${\scriptstyle\pm0.92}$ & 47.42${\scriptstyle\pm0.66}$ & 56.33${\scriptstyle\pm0.78}$ & 65.2${\scriptstyle\pm0.82}$ & 75.94${\scriptstyle\pm0.62}$ & 85.12${\scriptstyle\pm0.78}$ & 91.43${\scriptstyle\pm0.54}$ & 95.91${\scriptstyle\pm0.32}$ & 99.1${\scriptstyle\pm0.12}$  \\
% CPGNN & 18.59${\scriptstyle\pm1.61}$ & 20.51${\scriptstyle\pm0.95}$ & 20.26${\scriptstyle\pm0.85}$ & 18.77${\scriptstyle\pm1.9}$ & 20.2${\scriptstyle\pm1.81}$ & 20.91${\scriptstyle\pm1.03}$ & 19.97${\scriptstyle\pm1.17}$ & 19.7${\scriptstyle\pm1.56}$ & 20.12${\scriptstyle\pm1.1}$ & 19.87${\scriptstyle\pm0.8}$ & 21.12${\scriptstyle\pm1.07}$  \\
% LP & 9.52${\scriptstyle\pm0.85}$ & 10.02${\scriptstyle\pm0.33}$ & 14.78${\scriptstyle\pm0.39}$ & 20.58${\scriptstyle\pm0.53}$ & 29.73${\scriptstyle\pm0.58}$ & 40.8${\scriptstyle\pm0.72}$ & 55.19${\scriptstyle\pm0.55}$ & 73.27${\scriptstyle\pm0.65}$ & 86.07${\scriptstyle\pm0.43}$ & 95.59${\scriptstyle\pm0.22}$ & 99.39${\scriptstyle\pm0.04}$  \\
% C\&S & 38.86${\scriptstyle\pm4.79}$ & 38.47${\scriptstyle\pm4.18}$ & 40.88${\scriptstyle\pm2.5}$ & 42.2${\scriptstyle\pm1.75}$ & 50.36${\scriptstyle\pm1.39}$ & 60.46${\scriptstyle\pm1.84}$ & 73.65${\scriptstyle\pm1.54}$ & 88.08${\scriptstyle\pm0.44}$ & 94.57${\scriptstyle\pm0.32}$ & 98.19${\scriptstyle\pm0.18}$ & 99.54${\scriptstyle\pm0.1}$  \\
% CLP & 49.48${\scriptstyle\pm0.5}$ & 45.12${\scriptstyle\pm0.43}$ & 47.49${\scriptstyle\pm0.61}$ & 51.46${\scriptstyle\pm0.79}$ & 61.13${\scriptstyle\pm1.4}$ & 71.09${\scriptstyle\pm2.86}$ & 80.06${\scriptstyle\pm1.41}$ & 88.06${\scriptstyle\pm1.2}$ & 92.56${\scriptstyle\pm0.67}$ & 96.92${\scriptstyle\pm0.29}$ & 99.38${\scriptstyle\pm0.04}$  \\
% % \rowcolor{gray!30}
% % CLP\textsuperscript{\dag} & 48.93${\scriptstyle\pm0.45}$ & 45.18${\scriptstyle\pm0.42}$ & 47.32${\scriptstyle\pm0.44}$ & 55.23${\scriptstyle\pm0.79}$ & 60.58${\scriptstyle\pm2.04}$ & 67.99${\scriptstyle\pm0.92}$ & 80.88${\scriptstyle\pm0.57}$ & 90.29${\scriptstyle\pm0.5}$ & 94.34${\scriptstyle\pm0.24}$ & 97.53${\scriptstyle\pm0.23}$ & 99.6${\scriptstyle\pm0.03}$  \\
%         & \multicolumn{11}{c}{\textbf{Train ratio $48\%$}}  \\
% MLP & 44.98${\scriptstyle\pm1.03}$ & 44.88${\scriptstyle\pm0.77}$ & 45.82${\scriptstyle\pm0.67}$ & 45.12${\scriptstyle\pm1.11}$ & 47.36${\scriptstyle\pm1.21}$ & 46.25${\scriptstyle\pm1.2}$ & 45.19${\scriptstyle\pm0.7}$ & 46.44${\scriptstyle\pm0.79}$ & 44.96${\scriptstyle\pm0.95}$ & 44.47${\scriptstyle\pm1.18}$ & 45.54${\scriptstyle\pm0.67}$  \\
% GCN & 23.42${\scriptstyle\pm0.76}$ & 25.46${\scriptstyle\pm1.15}$ & 29.62${\scriptstyle\pm0.93}$ & 34.94${\scriptstyle\pm0.64}$ & 44.44${\scriptstyle\pm0.93}$ & 55.18${\scriptstyle\pm0.82}$ & 65.2${\scriptstyle\pm1.03}$ & 77.49${\scriptstyle\pm0.81}$ & 84.78${\scriptstyle\pm0.97}$ & 91.5${\scriptstyle\pm0.57}$ & 95.8${\scriptstyle\pm0.51}$  \\
% GAT & 28.22${\scriptstyle\pm1.36}$ & 29.2${\scriptstyle\pm1.74}$ & 33.83${\scriptstyle\pm0.85}$ & 38.48${\scriptstyle\pm0.89}$ & 46.95${\scriptstyle\pm1.42}$ & 56.3${\scriptstyle\pm0.99}$ & 65.22${\scriptstyle\pm0.97}$ & 76.22${\scriptstyle\pm1.03}$ & 83.58${\scriptstyle\pm0.96}$ & 91.4${\scriptstyle\pm0.5}$ & 97.71${\scriptstyle\pm0.51}$  \\
% GCN2 & 44.57${\scriptstyle\pm1.13}$ & 44.28${\scriptstyle\pm1.18}$ & 45.17${\scriptstyle\pm0.93}$ & 46.16${\scriptstyle\pm0.67}$ & 50.74${\scriptstyle\pm1.14}$ & 55.64${\scriptstyle\pm0.9}$ & 61.82${\scriptstyle\pm1.03}$ & 71.34${\scriptstyle\pm1.27}$ & 80.81${\scriptstyle\pm1.09}$ & 92.9${\scriptstyle\pm0.56}$ & 99.58${\scriptstyle\pm0.11}$  \\
% SuperGAT & 18.78${\scriptstyle\pm1.73}$ & 20.47${\scriptstyle\pm2.2}$ & 23.22${\scriptstyle\pm1.52}$ & 27.77${\scriptstyle\pm1.89}$ & 33.85${\scriptstyle\pm2.93}$ & 38.02${\scriptstyle\pm2.4}$ & 44.58${\scriptstyle\pm3.47}$ & 55.01${\scriptstyle\pm4.54}$ & 61.94${\scriptstyle\pm3.18}$ & 69.59${\scriptstyle\pm7.76}$ & 82.93${\scriptstyle\pm6.12}$  \\
% GPRGNN & 45.14${\scriptstyle\pm0.9}$ & 44.54${\scriptstyle\pm1.12}$ & 46.02${\scriptstyle\pm0.89}$ & 47.07${\scriptstyle\pm1.01}$ & 51.17${\scriptstyle\pm1.26}$ & 56.64${\scriptstyle\pm1.37}$ & 63.42${\scriptstyle\pm1.68}$ & 76.4${\scriptstyle\pm1.83}$ & 86.28${\scriptstyle\pm0.95}$ & 95.6${\scriptstyle\pm0.42}$ & 99.51${\scriptstyle\pm0.11}$  \\
% FAGCN & 45.22${\scriptstyle\pm1.14}$ & 45.02${\scriptstyle\pm0.79}$ & 46.01${\scriptstyle\pm0.66}$ & 46.99${\scriptstyle\pm1.03}$ & 50.38${\scriptstyle\pm1.55}$ & 53.5${\scriptstyle\pm2.34}$ & 58.6${\scriptstyle\pm3.04}$ & 67.18${\scriptstyle\pm3.67}$ & 74.29${\scriptstyle\pm4.4}$ & 83.08${\scriptstyle\pm3.78}$ & 90.6${\scriptstyle\pm2.55}$  \\
% H2GCN & 47.18${\scriptstyle\pm1.14}$ & 44.28${\scriptstyle\pm0.9}$ & 46.92${\scriptstyle\pm0.99}$ & 51.7${\scriptstyle\pm0.81}$ & 60.14${\scriptstyle\pm0.6}$ & 70.39${\scriptstyle\pm0.65}$ & 79.63${\scriptstyle\pm0.52}$ & 89.3${\scriptstyle\pm0.8}$ & 93.58${\scriptstyle\pm0.6}$ & 97.55${\scriptstyle\pm0.28}$ & 99.34${\scriptstyle\pm0.18}$  \\
% CPGNN & 19.94${\scriptstyle\pm0.78}$ & 19.76${\scriptstyle\pm1.26}$ & 19.55${\scriptstyle\pm0.86}$ & 19.55${\scriptstyle\pm1.29}$ & 19.92${\scriptstyle\pm0.99}$ & 21.57${\scriptstyle\pm0.88}$ & 20.56${\scriptstyle\pm1.58}$ & 21.28${\scriptstyle\pm0.56}$ & 19.49${\scriptstyle\pm0.9}$ & 19.21${\scriptstyle\pm1.68}$ & 21.2${\scriptstyle\pm0.79}$  \\
% LP & 9.3${\scriptstyle\pm0.45}$ & 10.51${\scriptstyle\pm0.73}$ & 21.68${\scriptstyle\pm0.76}$ & 33.88${\scriptstyle\pm1.03}$ & 48.05${\scriptstyle\pm1.02}$ & 62.21${\scriptstyle\pm0.72}$ & 75.41${\scriptstyle\pm0.85}$ & 86.86${\scriptstyle\pm0.5}$ & 93.12${\scriptstyle\pm0.53}$ & 97.65${\scriptstyle\pm0.31}$ & 99.38${\scriptstyle\pm0.15}$  \\
% C\&S & 38.39${\scriptstyle\pm4.45}$ & 39.62${\scriptstyle\pm2.93}$ & 45.33${\scriptstyle\pm1.33}$ & 55.9${\scriptstyle\pm1.8}$ & 67.18${\scriptstyle\pm1.34}$ & 77.45${\scriptstyle\pm0.65}$ & 86.03${\scriptstyle\pm0.59}$ & 93.28${\scriptstyle\pm0.69}$ & 96.51${\scriptstyle\pm0.47}$ & 98.64${\scriptstyle\pm0.19}$ & 99.58${\scriptstyle\pm0.13}$  \\
% CLP & 55.67${\scriptstyle\pm0.98}$ & 45.43${\scriptstyle\pm0.68}$ & 52.2${\scriptstyle\pm0.86}$ & 60.89${\scriptstyle\pm1.54}$ & 70.56${\scriptstyle\pm1.26}$ & 78.75${\scriptstyle\pm1.28}$ & 85.73${\scriptstyle\pm0.91}$ & 91.54${\scriptstyle\pm0.56}$ & 94.65${\scriptstyle\pm0.51}$ & 97.66${\scriptstyle\pm0.3}$ & 99.46${\scriptstyle\pm0.16}$  \\
% % \rowcolor{gray!30}
% % CLP\textsuperscript{\dag} & 55.7${\scriptstyle\pm1.33}$ & 45.74${\scriptstyle\pm0.71}$ & 51.84${\scriptstyle\pm0.77}$ & 65.62${\scriptstyle\pm0.95}$ & 68.88${\scriptstyle\pm1.05}$ & 78.54${\scriptstyle\pm1.1}$ & 87.03${\scriptstyle\pm0.62}$ & 93.64${\scriptstyle\pm0.35}$ & 96.24${\scriptstyle\pm0.26}$ & 98.54${\scriptstyle\pm0.2}$ & 99.59${\scriptstyle\pm0.13}$  \\
% \hline
% \end{tabular}
% }
% \end{table*}

% \begin{table*}
% \caption{Node classification results of Syn-2 dataset. 
% % \textsuperscript{\dag} means utilise spectral features.
% }
% % \vspace{-3mm}
% \label{table:NC_experimental_results_syn_self_010}
% % \small
% \centering
% \resizebox{.7\textwidth}{!}{
% \begin{tabular}{l ccccccccccc}
% \hline
% $h$     & 0.0 & 0.1 & 0.2 & 0.3 & 0.4 & 0.5 & 0.6 & 0.7 & 0.8 & 0.9 & 1.0 \\
%         & \multicolumn{11}{c}{\textbf{Train ratio $5\%$}}  \\
% MLP & 45.25${\scriptstyle\pm0.82}$ & 44.95${\scriptstyle\pm0.6}$ & 44.88${\scriptstyle\pm0.46}$ & 44.69${\scriptstyle\pm0.67}$ & 44.75${\scriptstyle\pm0.73}$ & 43.98${\scriptstyle\pm0.9}$ & 44.8${\scriptstyle\pm0.67}$ & 45.01${\scriptstyle\pm0.69}$ & 44.79${\scriptstyle\pm0.8}$ & 44.31${\scriptstyle\pm0.76}$ & 43.97${\scriptstyle\pm0.69}$  \\
% GCN & 24.23${\scriptstyle\pm0.54}$ & 24.44${\scriptstyle\pm0.54}$ & 29.3${\scriptstyle\pm0.75}$ & 36.77${\scriptstyle\pm0.95}$ & 50.45${\scriptstyle\pm1.44}$ & 67.17${\scriptstyle\pm1.24}$ & 81.34${\scriptstyle\pm0.94}$ & 91.01${\scriptstyle\pm0.86}$ & 96.23${\scriptstyle\pm0.4}$ & 98.67${\scriptstyle\pm0.39}$ & 99.7${\scriptstyle\pm0.17}$  \\
% GAT & 26.97${\scriptstyle\pm1.39}$ & 25.31${\scriptstyle\pm2.14}$ & 31.03${\scriptstyle\pm1.75}$ & 39.27${\scriptstyle\pm2.19}$ & 53.12${\scriptstyle\pm1.76}$ & 67.36${\scriptstyle\pm2.16}$ & 80.03${\scriptstyle\pm1.3}$ & 90.39${\scriptstyle\pm1.23}$ & 95.92${\scriptstyle\pm0.53}$ & 98.72${\scriptstyle\pm0.38}$ & 99.75${\scriptstyle\pm0.17}$  \\
% GCN2 & 15.59${\scriptstyle\pm11.26}$ & 16.01${\scriptstyle\pm12.03}$ & 16.45${\scriptstyle\pm12.98}$ & 17.3${\scriptstyle\pm14.75}$ & 18.45${\scriptstyle\pm16.86}$ & 20.01${\scriptstyle\pm19.99}$ & 21.83${\scriptstyle\pm23.76}$ & 23.79${\scriptstyle\pm27.62}$ & 25.97${\scriptstyle\pm31.94}$ & 27.63${\scriptstyle\pm35.21}$ & 27.94${\scriptstyle\pm35.98}$  \\
% SuperGAT & 17.39${\scriptstyle\pm1.84}$ & 17.05${\scriptstyle\pm2.53}$ & 20.72${\scriptstyle\pm1.91}$ & 24.42${\scriptstyle\pm2.56}$ & 30.02${\scriptstyle\pm3.0}$ & 34.69${\scriptstyle\pm3.2}$ & 40.21${\scriptstyle\pm4.41}$ & 44.59${\scriptstyle\pm5.0}$ & 49.41${\scriptstyle\pm7.06}$ & 55.4${\scriptstyle\pm6.75}$ & 62.99${\scriptstyle\pm9.39}$  \\
% GPRGNN & 43.87${\scriptstyle\pm1.78}$ & 42.82${\scriptstyle\pm1.6}$ & 43.51${\scriptstyle\pm1.45}$ & 45.09${\scriptstyle\pm1.8}$ & 51.06${\scriptstyle\pm2.26}$ & 61.39${\scriptstyle\pm3.72}$ & 73.11${\scriptstyle\pm3.07}$ & 85.77${\scriptstyle\pm2.33}$ & 94.86${\scriptstyle\pm0.96}$ & 98.61${\scriptstyle\pm0.43}$ & 99.86${\scriptstyle\pm0.13}$  \\
% FAGCN & 45.92${\scriptstyle\pm0.83}$ & 44.95${\scriptstyle\pm0.94}$ & 45.79${\scriptstyle\pm0.63}$ & 47.68${\scriptstyle\pm1.27}$ & 53.51${\scriptstyle\pm2.61}$ & 61.93${\scriptstyle\pm5.45}$ & 71.62${\scriptstyle\pm6.68}$ & 82.04${\scriptstyle\pm6.75}$ & 89.81${\scriptstyle\pm4.04}$ & 95.49${\scriptstyle\pm2.07}$ & 97.72${\scriptstyle\pm1.2}$  \\
% H2GCN & 43.04${\scriptstyle\pm1.02}$ & 40.5${\scriptstyle\pm1.32}$ & 42.28${\scriptstyle\pm1.24}$ & 49.25${\scriptstyle\pm1.43}$ & 62.69${\scriptstyle\pm1.63}$ & 77.67${\scriptstyle\pm1.39}$ & 88.04${\scriptstyle\pm1.24}$ & 94.93${\scriptstyle\pm0.6}$ & 97.89${\scriptstyle\pm0.36}$ & 99.34${\scriptstyle\pm0.21}$ & 99.79${\scriptstyle\pm0.21}$  \\
% CPGNN & 20.13${\scriptstyle\pm1.57}$ & 20.65${\scriptstyle\pm0.78}$ & 20.02${\scriptstyle\pm1.64}$ & 20.06${\scriptstyle\pm0.91}$ & 20.95${\scriptstyle\pm2.17}$ & 22.47${\scriptstyle\pm2.74}$ & 22.87${\scriptstyle\pm4.11}$ & 20.43${\scriptstyle\pm1.77}$ & 20.58${\scriptstyle\pm1.01}$ & 20.21${\scriptstyle\pm1.72}$ & 19.92${\scriptstyle\pm1.7}$  \\
% LP & 9.79${\scriptstyle\pm0.56}$ & 9.89${\scriptstyle\pm0.24}$ & 15.21${\scriptstyle\pm0.38}$ & 22.4${\scriptstyle\pm0.46}$ & 32.99${\scriptstyle\pm0.87}$ & 48.05${\scriptstyle\pm1.25}$ & 67.35${\scriptstyle\pm1.38}$ & 83.84${\scriptstyle\pm0.89}$ & 93.57${\scriptstyle\pm0.45}$ & 98.82${\scriptstyle\pm0.14}$ & 100.0${\scriptstyle\pm0.01}$  \\
% C\&S & 40.99${\scriptstyle\pm3.88}$ & 40.26${\scriptstyle\pm4.28}$ & 40.92${\scriptstyle\pm2.89}$ & 44.61${\scriptstyle\pm1.92}$ & 54.04${\scriptstyle\pm1.9}$ & 70.77${\scriptstyle\pm2.07}$ & 87.3${\scriptstyle\pm1.42}$ & 96.62${\scriptstyle\pm0.81}$ & 99.4${\scriptstyle\pm0.16}$ & 99.78${\scriptstyle\pm0.14}$ & 99.94${\scriptstyle\pm0.1}$  \\
% CLP & 51.12${\scriptstyle\pm0.76}$ & 44.93${\scriptstyle\pm0.69}$ & 47.84${\scriptstyle\pm1.07}$ & 55.3${\scriptstyle\pm1.51}$ & 68.02${\scriptstyle\pm2.4}$ & 79.47${\scriptstyle\pm2.01}$ & 86.77${\scriptstyle\pm1.65}$ & 92.36${\scriptstyle\pm1.52}$ & 95.56${\scriptstyle\pm1.37}$ & 98.5${\scriptstyle\pm0.61}$ & 100.0${\scriptstyle\pm0.0}$  \\
% % \rowcolor{gray!30}
% % CLP\textsuperscript{\dag} & 50.57${\scriptstyle\pm0.87}$ & 45.22${\scriptstyle\pm0.6}$ & 47.85${\scriptstyle\pm1.06}$ & 55.38${\scriptstyle\pm1.61}$ & 66.04${\scriptstyle\pm2.07}$ & 82.14${\scriptstyle\pm1.37}$ & 89.81${\scriptstyle\pm0.76}$ & 94.27${\scriptstyle\pm0.54}$ & 98.3${\scriptstyle\pm0.4}$ & 99.82${\scriptstyle\pm0.06}$ & 100.0${\scriptstyle\pm0.0}$  \\
%         & \multicolumn{11}{c}{\textbf{Train ratio $10\%$}}  \\
% MLP & 45.45${\scriptstyle\pm0.61}$ & 45.65${\scriptstyle\pm0.45}$ & 45.22${\scriptstyle\pm0.49}$ & 44.98${\scriptstyle\pm0.57}$ & 45.24${\scriptstyle\pm0.52}$ & 44.69${\scriptstyle\pm0.55}$ & 45.08${\scriptstyle\pm0.5}$ & 45.55${\scriptstyle\pm0.57}$ & 45.5${\scriptstyle\pm0.54}$ & 44.96${\scriptstyle\pm0.54}$ & 44.54${\scriptstyle\pm0.56}$  \\
% GCN & 24.77${\scriptstyle\pm0.57}$ & 24.81${\scriptstyle\pm0.67}$ & 29.97${\scriptstyle\pm0.54}$ & 37.55${\scriptstyle\pm0.97}$ & 52.43${\scriptstyle\pm0.83}$ & 68.89${\scriptstyle\pm1.08}$ & 82.42${\scriptstyle\pm0.66}$ & 92.57${\scriptstyle\pm0.54}$ & 96.71${\scriptstyle\pm0.42}$ & 98.9${\scriptstyle\pm0.22}$ & 99.85${\scriptstyle\pm0.08}$  \\
% GAT & 28.58${\scriptstyle\pm1.1}$ & 26.98${\scriptstyle\pm1.78}$ & 32.53${\scriptstyle\pm1.62}$ & 41.89${\scriptstyle\pm1.71}$ & 55.82${\scriptstyle\pm1.47}$ & 69.8${\scriptstyle\pm1.29}$ & 81.85${\scriptstyle\pm1.35}$ & 91.75${\scriptstyle\pm0.92}$ & 96.48${\scriptstyle\pm0.45}$ & 99.0${\scriptstyle\pm0.17}$ & 99.85${\scriptstyle\pm0.09}$  \\
% GCN2 & 16.55${\scriptstyle\pm13.05}$ & 16.44${\scriptstyle\pm12.76}$ & 16.8${\scriptstyle\pm13.68}$ & 17.64${\scriptstyle\pm15.38}$ & 18.92${\scriptstyle\pm17.83}$ & 20.15${\scriptstyle\pm20.41}$ & 22.07${\scriptstyle\pm24.27}$ & 23.96${\scriptstyle\pm27.82}$ & 26.03${\scriptstyle\pm32.2}$ & 27.64${\scriptstyle\pm35.34}$ & 27.98${\scriptstyle\pm35.98}$  \\
% SuperGAT & 17.14${\scriptstyle\pm2.37}$ & 17.64${\scriptstyle\pm2.22}$ & 20.76${\scriptstyle\pm1.85}$ & 23.2${\scriptstyle\pm2.24}$ & 30.33${\scriptstyle\pm3.56}$ & 36.28${\scriptstyle\pm3.4}$ & 43.94${\scriptstyle\pm7.43}$ & 49.46${\scriptstyle\pm5.33}$ & 58.44${\scriptstyle\pm6.25}$ & 58.79${\scriptstyle\pm8.57}$ & 67.59${\scriptstyle\pm9.12}$  \\
% GPRGNN & 45.07${\scriptstyle\pm1.07}$ & 44.3${\scriptstyle\pm0.93}$ & 44.33${\scriptstyle\pm1.31}$ & 46.76${\scriptstyle\pm1.55}$ & 54.11${\scriptstyle\pm1.93}$ & 64.76${\scriptstyle\pm2.54}$ & 74.15${\scriptstyle\pm2.72}$ & 86.34${\scriptstyle\pm1.76}$ & 95.22${\scriptstyle\pm0.72}$ & 98.9${\scriptstyle\pm0.21}$ & 99.94${\scriptstyle\pm0.06}$  \\
% FAGCN & 46.29${\scriptstyle\pm0.67}$ & 45.65${\scriptstyle\pm0.52}$ & 46.22${\scriptstyle\pm0.52}$ & 48.56${\scriptstyle\pm1.14}$ & 53.96${\scriptstyle\pm2.48}$ & 63.04${\scriptstyle\pm5.65}$ & 73.78${\scriptstyle\pm6.89}$ & 83.33${\scriptstyle\pm6.17}$ & 91.81${\scriptstyle\pm3.67}$ & 96.04${\scriptstyle\pm1.72}$ & 98.9${\scriptstyle\pm0.56}$  \\
% H2GCN & 45.73${\scriptstyle\pm0.9}$ & 41.79${\scriptstyle\pm0.9}$ & 44.55${\scriptstyle\pm0.9}$ & 53.01${\scriptstyle\pm0.97}$ & 66.52${\scriptstyle\pm1.39}$ & 80.76${\scriptstyle\pm1.79}$ & 90.5${\scriptstyle\pm1.08}$ & 96.01${\scriptstyle\pm0.61}$ & 98.41${\scriptstyle\pm0.27}$ & 99.53${\scriptstyle\pm0.12}$ & 99.94${\scriptstyle\pm0.06}$  \\
% CPGNN & 20.58${\scriptstyle\pm0.83}$ & 20.31${\scriptstyle\pm0.92}$ & 20.25${\scriptstyle\pm0.92}$ & 20.23${\scriptstyle\pm0.88}$ & 21.79${\scriptstyle\pm1.62}$ & 22.41${\scriptstyle\pm2.22}$ & 22.86${\scriptstyle\pm4.21}$ & 20.11${\scriptstyle\pm1.06}$ & 20.2${\scriptstyle\pm1.24}$ & 20.17${\scriptstyle\pm1.08}$ & 19.45${\scriptstyle\pm1.13}$  \\
% LP & 9.85${\scriptstyle\pm0.13}$ & 9.95${\scriptstyle\pm0.32}$ & 17.56${\scriptstyle\pm0.41}$ & 27.11${\scriptstyle\pm0.43}$ & 40.61${\scriptstyle\pm0.92}$ & 56.67${\scriptstyle\pm0.91}$ & 74.03${\scriptstyle\pm0.9}$ & 87.64${\scriptstyle\pm0.65}$ & 96.43${\scriptstyle\pm0.17}$ & 99.65${\scriptstyle\pm0.06}$ & 100.0${\scriptstyle\pm0.0}$  \\
% C\&S & 40.3${\scriptstyle\pm4.59}$ & 40.32${\scriptstyle\pm4.38}$ & 40.93${\scriptstyle\pm3.13}$ & 48.8${\scriptstyle\pm2.13}$ & 61.79${\scriptstyle\pm1.51}$ & 78.43${\scriptstyle\pm1.4}$ & 91.51${\scriptstyle\pm1.0}$ & 97.95${\scriptstyle\pm0.34}$ & 99.62${\scriptstyle\pm0.1}$ & 99.89${\scriptstyle\pm0.07}$ & 99.98${\scriptstyle\pm0.04}$  \\
% CLP & 53.54${\scriptstyle\pm0.76}$ & 45.66${\scriptstyle\pm0.46}$ & 49.88${\scriptstyle\pm0.91}$ & 60.68${\scriptstyle\pm1.67}$ & 72.92${\scriptstyle\pm1.53}$ & 82.95${\scriptstyle\pm2.09}$ & 89.95${\scriptstyle\pm1.93}$ & 94.23${\scriptstyle\pm1.3}$ & 96.58${\scriptstyle\pm1.02}$ & 98.8${\scriptstyle\pm0.3}$ & 100.0${\scriptstyle\pm0.0}$  \\
% % \rowcolor{gray!30}
% % CLP\textsuperscript{\dag} & 52.98${\scriptstyle\pm0.71}$ & 45.58${\scriptstyle\pm0.54}$ & 49.81${\scriptstyle\pm0.83}$ & 58.7${\scriptstyle\pm2.69}$ & 72.19${\scriptstyle\pm0.66}$ & 87.71${\scriptstyle\pm0.52}$ & 93.94${\scriptstyle\pm0.59}$ & 96.43${\scriptstyle\pm0.37}$ & 98.28${\scriptstyle\pm0.19}$ & 99.86${\scriptstyle\pm0.05}$ & 100.0${\scriptstyle\pm0.0}$  \\
%         & \multicolumn{11}{c}{\textbf{Train ratio $48\%$}}  \\
% MLP & 46.24${\scriptstyle\pm0.87}$ & 45.83${\scriptstyle\pm0.85}$ & 45.74${\scriptstyle\pm0.81}$ & 45.41${\scriptstyle\pm0.98}$ & 45.45${\scriptstyle\pm1.0}$ & 45.52${\scriptstyle\pm1.04}$ & 45.81${\scriptstyle\pm1.08}$ & 45.9${\scriptstyle\pm0.89}$ & 46.02${\scriptstyle\pm1.06}$ & 46.06${\scriptstyle\pm1.42}$ & 45.5${\scriptstyle\pm0.92}$  \\
% GCN & 25.24${\scriptstyle\pm0.67}$ & 25.5${\scriptstyle\pm0.87}$ & 30.84${\scriptstyle\pm1.11}$ & 39.31${\scriptstyle\pm1.41}$ & 53.9${\scriptstyle\pm1.01}$ & 70.59${\scriptstyle\pm1.11}$ & 83.64${\scriptstyle\pm0.83}$ & 93.48${\scriptstyle\pm0.56}$ & 97.48${\scriptstyle\pm0.33}$ & 99.0${\scriptstyle\pm0.23}$ & 99.88${\scriptstyle\pm0.06}$  \\
% GAT & 30.42${\scriptstyle\pm1.3}$ & 29.09${\scriptstyle\pm1.27}$ & 35.99${\scriptstyle\pm1.27}$ & 44.98${\scriptstyle\pm1.06}$ & 58.27${\scriptstyle\pm1.41}$ & 72.22${\scriptstyle\pm1.24}$ & 83.71${\scriptstyle\pm0.85}$ & 92.85${\scriptstyle\pm0.84}$ & 97.21${\scriptstyle\pm0.42}$ & 99.15${\scriptstyle\pm0.2}$ & 99.93${\scriptstyle\pm0.06}$  \\
% GCN2 & 17.1${\scriptstyle\pm14.05}$ & 16.57${\scriptstyle\pm14.02}$ & 17.13${\scriptstyle\pm14.46}$ & 17.68${\scriptstyle\pm16.42}$ & 19.13${\scriptstyle\pm18.1}$ & 20.48${\scriptstyle\pm20.54}$ & 21.95${\scriptstyle\pm24.66}$ & 24.01${\scriptstyle\pm28.13}$ & 26.5${\scriptstyle\pm32.31}$ & 27.47${\scriptstyle\pm35.51}$ & 27.81${\scriptstyle\pm36.09}$  \\
% SuperGAT & 18.9${\scriptstyle\pm1.65}$ & 20.38${\scriptstyle\pm1.55}$ & 23.72${\scriptstyle\pm2.0}$ & 28.84${\scriptstyle\pm2.68}$ & 37.98${\scriptstyle\pm3.27}$ & 46.43${\scriptstyle\pm6.1}$ & 56.44${\scriptstyle\pm5.48}$ & 61.18${\scriptstyle\pm6.21}$ & 68.86${\scriptstyle\pm5.16}$ & 81.42${\scriptstyle\pm6.23}$ & 87.93${\scriptstyle\pm7.16}$  \\
% GPRGNN & 46.27${\scriptstyle\pm1.09}$ & 45.17${\scriptstyle\pm1.1}$ & 45.95${\scriptstyle\pm1.23}$ & 48.59${\scriptstyle\pm1.29}$ & 55.6${\scriptstyle\pm1.93}$ & 65.35${\scriptstyle\pm2.79}$ & 74.45${\scriptstyle\pm2.99}$ & 87.23${\scriptstyle\pm1.62}$ & 95.47${\scriptstyle\pm0.86}$ & 99.02${\scriptstyle\pm0.23}$ & 99.98${\scriptstyle\pm0.03}$  \\
% FAGCN & 46.71${\scriptstyle\pm0.95}$ & 45.99${\scriptstyle\pm0.89}$ & 46.78${\scriptstyle\pm1.05}$ & 48.65${\scriptstyle\pm1.75}$ & 55.35${\scriptstyle\pm2.68}$ & 64.26${\scriptstyle\pm6.59}$ & 75.3${\scriptstyle\pm6.24}$ & 86.53${\scriptstyle\pm4.88}$ & 92.88${\scriptstyle\pm3.21}$ & 97.19${\scriptstyle\pm1.36}$ & 99.34${\scriptstyle\pm0.49}$  \\
% H2GCN & 50.01${\scriptstyle\pm0.9}$ & 44.44${\scriptstyle\pm1.26}$ & 49.15${\scriptstyle\pm1.04}$ & 57.34${\scriptstyle\pm1.25}$ & 71.54${\scriptstyle\pm1.23}$ & 85.66${\scriptstyle\pm1.26}$ & 93.2${\scriptstyle\pm0.88}$ & 97.49${\scriptstyle\pm0.48}$ & 99.15${\scriptstyle\pm0.26}$ & 99.67${\scriptstyle\pm0.12}$ & 99.98${\scriptstyle\pm0.03}$  \\
% CPGNN & 20.91${\scriptstyle\pm1.24}$ & 19.84${\scriptstyle\pm1.16}$ & 20.39${\scriptstyle\pm1.67}$ & 20.38${\scriptstyle\pm0.87}$ & 22.08${\scriptstyle\pm1.67}$ & 22.82${\scriptstyle\pm2.69}$ & 23.69${\scriptstyle\pm3.68}$ & 20.19${\scriptstyle\pm1.27}$ & 20.12${\scriptstyle\pm0.96}$ & 19.05${\scriptstyle\pm1.82}$ & 19.33${\scriptstyle\pm0.99}$  \\
% LP & 9.51${\scriptstyle\pm0.6}$ & 9.62${\scriptstyle\pm0.67}$ & 27.18${\scriptstyle\pm0.96}$ & 46.86${\scriptstyle\pm1.25}$ & 66.53${\scriptstyle\pm1.08}$ & 82.28${\scriptstyle\pm0.89}$ & 92.83${\scriptstyle\pm0.5}$ & 97.82${\scriptstyle\pm0.29}$ & 99.5${\scriptstyle\pm0.15}$ & 99.88${\scriptstyle\pm0.08}$ & 100.0${\scriptstyle\pm0.0}$  \\
% C\&S & 38.81${\scriptstyle\pm4.89}$ & 40.11${\scriptstyle\pm2.74}$ & 53.45${\scriptstyle\pm1.35}$ & 67.63${\scriptstyle\pm1.34}$ & 81.6${\scriptstyle\pm1.2}$ & 91.96${\scriptstyle\pm0.88}$ & 97.16${\scriptstyle\pm0.35}$ & 99.13${\scriptstyle\pm0.23}$ & 99.83${\scriptstyle\pm0.08}$ & 99.93${\scriptstyle\pm0.07}$ & 100.0${\scriptstyle\pm0.01}$  \\
% CLP & 65.23${\scriptstyle\pm1.17}$ & 45.58${\scriptstyle\pm0.91}$ & 57.58${\scriptstyle\pm1.41}$ & 70.8${\scriptstyle\pm1.23}$ & 81.25${\scriptstyle\pm1.3}$ & 88.23${\scriptstyle\pm1.52}$ & 93.86${\scriptstyle\pm0.95}$ & 96.17${\scriptstyle\pm0.77}$ & 97.91${\scriptstyle\pm0.52}$ & 99.22${\scriptstyle\pm0.3}$ & 100.0${\scriptstyle\pm0.0}$  \\
% % \rowcolor{gray!30}
% % CLP\textsuperscript{\dag} & 64.5${\scriptstyle\pm1.08}$ & 45.67${\scriptstyle\pm0.86}$ & 57.23${\scriptstyle\pm1.23}$ & 68.96${\scriptstyle\pm0.92}$ & 82.75${\scriptstyle\pm0.7}$ & 92.75${\scriptstyle\pm0.61}$ & 97.0${\scriptstyle\pm0.32}$ & 98.95${\scriptstyle\pm0.21}$ & 99.07${\scriptstyle\pm0.23}$ & 99.84${\scriptstyle\pm0.11}$ & 100.0${\scriptstyle\pm0.0}$  \\
% \hline
% \end{tabular}
% }
% \end{table*}

% \begin{table*}
% \caption{Node classification results of Syn-3 dataset. 
% % \textsuperscript{\dag} means utilise spectral features.
% }
% % \vspace{-3mm}
% \label{table:NC_experimental_results_syn_self_015}
% % \small
% \centering
% \resizebox{.7\textwidth}{!}{
% \begin{tabular}{l ccccccccccc}
% \hline
% $h$     & 0.0 & 0.1 & 0.2 & 0.3 & 0.4 & 0.5 & 0.6 & 0.7 & 0.8 & 0.9 & 1.0\\
%         & \multicolumn{11}{c}{\textbf{Train ratio $5\%$}}  \\
% MLP & 44.5${\scriptstyle\pm0.62}$ & 44.89${\scriptstyle\pm0.77}$ & 44.0${\scriptstyle\pm0.76}$ & 45.33${\scriptstyle\pm0.47}$ & 44.55${\scriptstyle\pm0.73}$ & 44.57${\scriptstyle\pm0.73}$ & 44.02${\scriptstyle\pm0.62}$ & 44.58${\scriptstyle\pm0.66}$ & 45.64${\scriptstyle\pm0.73}$ & 45.49${\scriptstyle\pm0.48}$ & 44.29${\scriptstyle\pm0.92}$  \\
% GCN & 25.68${\scriptstyle\pm0.9}$ & 23.89${\scriptstyle\pm1.54}$ & 29.37${\scriptstyle\pm0.78}$ & 41.23${\scriptstyle\pm1.73}$ & 61.68${\scriptstyle\pm1.49}$ & 79.1${\scriptstyle\pm0.94}$ & 91.42${\scriptstyle\pm0.85}$ & 96.13${\scriptstyle\pm0.51}$ & 98.8${\scriptstyle\pm0.23}$ & 99.7${\scriptstyle\pm0.14}$ & 99.88${\scriptstyle\pm0.09}$  \\
% GAT & 27.75${\scriptstyle\pm1.64}$ & 25.67${\scriptstyle\pm1.76}$ & 31.12${\scriptstyle\pm1.26}$ & 44.95${\scriptstyle\pm2.36}$ & 62.75${\scriptstyle\pm2.18}$ & 77.84${\scriptstyle\pm1.47}$ & 89.39${\scriptstyle\pm1.33}$ & 95.59${\scriptstyle\pm0.54}$ & 98.68${\scriptstyle\pm0.27}$ & 99.62${\scriptstyle\pm0.23}$ & 99.84${\scriptstyle\pm0.15}$  \\
% GCN2 & 38.01${\scriptstyle\pm1.49}$ & 39.86${\scriptstyle\pm1.39}$ & 42.97${\scriptstyle\pm1.26}$ & 49.3${\scriptstyle\pm1.48}$ & 54.79${\scriptstyle\pm1.18}$ & 61.7${\scriptstyle\pm1.64}$ & 72.09${\scriptstyle\pm1.47}$ & 82.03${\scriptstyle\pm1.15}$ & 93.7${\scriptstyle\pm0.53}$ & 99.24${\scriptstyle\pm0.2}$ & 99.89${\scriptstyle\pm0.1}$  \\
% SuperGAT & 16.75${\scriptstyle\pm2.46}$ & 16.68${\scriptstyle\pm2.59}$ & 19.95${\scriptstyle\pm1.55}$ & 26.09${\scriptstyle\pm3.61}$ & 27.79${\scriptstyle\pm3.22}$ & 37.73${\scriptstyle\pm6.03}$ & 42.34${\scriptstyle\pm4.57}$ & 47.69${\scriptstyle\pm7.85}$ & 49.45${\scriptstyle\pm8.24}$ & 57.52${\scriptstyle\pm10.63}$ & 60.7${\scriptstyle\pm9.84}$  \\
% GPRGNN & 43.62${\scriptstyle\pm1.29}$ & 42.58${\scriptstyle\pm1.36}$ & 43.49${\scriptstyle\pm1.62}$ & 48.64${\scriptstyle\pm2.64}$ & 61.68${\scriptstyle\pm2.96}$ & 76.43${\scriptstyle\pm3.92}$ & 85.53${\scriptstyle\pm3.29}$ & 91.82${\scriptstyle\pm2.18}$ & 97.44${\scriptstyle\pm0.6}$ & 99.61${\scriptstyle\pm0.16}$ & 99.94${\scriptstyle\pm0.09}$  \\
% FAGCN & 45.57${\scriptstyle\pm0.54}$ & 44.62${\scriptstyle\pm1.05}$ & 45.39${\scriptstyle\pm0.98}$ & 50.29${\scriptstyle\pm1.8}$ & 60.61${\scriptstyle\pm4.31}$ & 73.29${\scriptstyle\pm4.45}$ & 82.05${\scriptstyle\pm6.63}$ & 89.02${\scriptstyle\pm6.14}$ & 96.17${\scriptstyle\pm1.97}$ & 98.33${\scriptstyle\pm0.94}$ & 99.08${\scriptstyle\pm0.43}$  \\
% H2GCN & 43.76${\scriptstyle\pm1.35}$ & 39.37${\scriptstyle\pm1.48}$ & 42.59${\scriptstyle\pm1.13}$ & 54.52${\scriptstyle\pm1.49}$ & 70.97${\scriptstyle\pm2.36}$ & 85.73${\scriptstyle\pm1.88}$ & 94.21${\scriptstyle\pm1.02}$ & 97.9${\scriptstyle\pm0.45}$ & 99.31${\scriptstyle\pm0.22}$ & 99.83${\scriptstyle\pm0.11}$ & 99.84${\scriptstyle\pm0.13}$  \\
% CPGNN & 20.09${\scriptstyle\pm1.5}$ & 20.24${\scriptstyle\pm1.32}$ & 19.82${\scriptstyle\pm1.29}$ & 21.57${\scriptstyle\pm1.78}$ & 21.86${\scriptstyle\pm2.69}$ & 22.91${\scriptstyle\pm3.87}$ & 23.95${\scriptstyle\pm5.66}$ & 27.32${\scriptstyle\pm6.66}$ & 29.3${\scriptstyle\pm8.93}$ & 29.1${\scriptstyle\pm9.99}$ & 30.38${\scriptstyle\pm12.0}$  \\
% LP & 9.9${\scriptstyle\pm0.09}$ & 9.96${\scriptstyle\pm0.22}$ & 16.24${\scriptstyle\pm0.29}$ & 26.01${\scriptstyle\pm0.57}$ & 40.21${\scriptstyle\pm0.86}$ & 58.05${\scriptstyle\pm2.24}$ & 75.48${\scriptstyle\pm1.41}$ & 87.1${\scriptstyle\pm0.58}$ & 96.16${\scriptstyle\pm0.33}$ & 99.78${\scriptstyle\pm0.08}$ & 99.99${\scriptstyle\pm0.01}$  \\
% C\&S & 40.97${\scriptstyle\pm3.09}$ & 38.86${\scriptstyle\pm4.83}$ & 40.26${\scriptstyle\pm3.02}$ & 48.38${\scriptstyle\pm2.22}$ & 62.0${\scriptstyle\pm1.77}$ & 78.89${\scriptstyle\pm2.42}$ & 92.99${\scriptstyle\pm1.23}$ & 98.72${\scriptstyle\pm0.39}$ & 99.81${\scriptstyle\pm0.15}$ & 99.91${\scriptstyle\pm0.11}$ & 99.95${\scriptstyle\pm0.08}$  \\
% CLP & 44.82${\scriptstyle\pm0.54}$ & 44.97${\scriptstyle\pm0.64}$ & 46.78${\scriptstyle\pm1.28}$ & 59.12${\scriptstyle\pm1.73}$ & 70.81${\scriptstyle\pm1.47}$ & 80.87${\scriptstyle\pm2.72}$ & 86.12${\scriptstyle\pm1.95}$ & 91.7${\scriptstyle\pm1.92}$ & 94.94${\scriptstyle\pm1.14}$ & 97.78${\scriptstyle\pm0.67}$ & 100.0${\scriptstyle\pm0.0}$  \\
% % \rowcolor{gray!30}
% % CLP\textsuperscript{\dag} & 53.19${\scriptstyle\pm1.1}$ & 45.54${\scriptstyle\pm0.64}$ & 47.71${\scriptstyle\pm1.58}$ & 59.13${\scriptstyle\pm2.9}$ & 76.75${\scriptstyle\pm1.24}$ & 88.36${\scriptstyle\pm1.28}$ & 93.36${\scriptstyle\pm0.39}$ & 96.69${\scriptstyle\pm0.39}$ & 99.46${\scriptstyle\pm0.2}$ & 99.99${\scriptstyle\pm0.01}$ & 100.0${\scriptstyle\pm0.0}$  \\
%         & \multicolumn{11}{c}{\textbf{Train ratio $10\%$}}  \\
% MLP & 45.16${\scriptstyle\pm0.43}$ & 45.41${\scriptstyle\pm0.42}$ & 44.44${\scriptstyle\pm0.64}$ & 45.77${\scriptstyle\pm0.46}$ & 44.97${\scriptstyle\pm0.38}$ & 45.24${\scriptstyle\pm0.47}$ & 44.55${\scriptstyle\pm0.62}$ & 44.94${\scriptstyle\pm0.59}$ & 46.02${\scriptstyle\pm0.42}$ & 45.53${\scriptstyle\pm0.61}$ & 44.88${\scriptstyle\pm0.47}$  \\
% GCN & 26.54${\scriptstyle\pm0.56}$ & 24.78${\scriptstyle\pm0.54}$ & 29.62${\scriptstyle\pm0.72}$ & 43.13${\scriptstyle\pm1.89}$ & 63.35${\scriptstyle\pm0.99}$ & 80.39${\scriptstyle\pm0.37}$ & 92.57${\scriptstyle\pm0.31}$ & 96.97${\scriptstyle\pm0.34}$ & 99.11${\scriptstyle\pm0.15}$ & 99.74${\scriptstyle\pm0.13}$ & 99.96${\scriptstyle\pm0.07}$  \\
% GAT & 29.88${\scriptstyle\pm0.93}$ & 27.71${\scriptstyle\pm1.29}$ & 32.41${\scriptstyle\pm1.58}$ & 47.29${\scriptstyle\pm1.96}$ & 65.32${\scriptstyle\pm1.66}$ & 79.44${\scriptstyle\pm1.67}$ & 90.93${\scriptstyle\pm0.65}$ & 96.53${\scriptstyle\pm0.4}$ & 99.12${\scriptstyle\pm0.21}$ & 99.83${\scriptstyle\pm0.06}$ & 99.96${\scriptstyle\pm0.03}$  \\
% GCN2 & 41.44${\scriptstyle\pm1.3}$ & 42.27${\scriptstyle\pm0.99}$ & 44.7${\scriptstyle\pm1.05}$ & 50.52${\scriptstyle\pm1.74}$ & 56.71${\scriptstyle\pm0.74}$ & 63.34${\scriptstyle\pm0.9}$ & 73.77${\scriptstyle\pm0.54}$ & 83.11${\scriptstyle\pm0.63}$ & 94.19${\scriptstyle\pm0.47}$ & 99.42${\scriptstyle\pm0.07}$ & 99.97${\scriptstyle\pm0.04}$  \\
% SuperGAT & 17.09${\scriptstyle\pm2.26}$ & 17.31${\scriptstyle\pm1.66}$ & 22.04${\scriptstyle\pm2.42}$ & 26.54${\scriptstyle\pm2.41}$ & 33.98${\scriptstyle\pm4.85}$ & 39.55${\scriptstyle\pm4.68}$ & 47.22${\scriptstyle\pm6.93}$ & 51.71${\scriptstyle\pm6.16}$ & 52.08${\scriptstyle\pm5.13}$ & 59.6${\scriptstyle\pm8.19}$ & 66.72${\scriptstyle\pm7.65}$  \\
% GPRGNN & 44.98${\scriptstyle\pm0.87}$ & 43.87${\scriptstyle\pm1.04}$ & 44.81${\scriptstyle\pm1.44}$ & 51.5${\scriptstyle\pm2.02}$ & 65.04${\scriptstyle\pm1.9}$ & 79.9${\scriptstyle\pm2.71}$ & 87.93${\scriptstyle\pm2.7}$ & 93.26${\scriptstyle\pm1.82}$ & 98.06${\scriptstyle\pm0.58}$ & 99.71${\scriptstyle\pm0.11}$ & 99.97${\scriptstyle\pm0.03}$  \\
% FAGCN & 46.24${\scriptstyle\pm0.6}$ & 45.38${\scriptstyle\pm0.61}$ & 46.09${\scriptstyle\pm0.71}$ & 51.43${\scriptstyle\pm1.33}$ & 62.21${\scriptstyle\pm4.35}$ & 71.81${\scriptstyle\pm6.31}$ & 82.71${\scriptstyle\pm7.35}$ & 88.96${\scriptstyle\pm5.12}$ & 97.39${\scriptstyle\pm1.89}$ & 99.0${\scriptstyle\pm0.69}$ & 99.65${\scriptstyle\pm0.15}$  \\
% H2GCN & 45.87${\scriptstyle\pm1.3}$ & 41.27${\scriptstyle\pm0.85}$ & 44.77${\scriptstyle\pm1.14}$ & 58.47${\scriptstyle\pm1.12}$ & 75.68${\scriptstyle\pm1.66}$ & 88.74${\scriptstyle\pm0.91}$ & 95.87${\scriptstyle\pm0.62}$ & 98.62${\scriptstyle\pm0.22}$ & 99.5${\scriptstyle\pm0.12}$ & 99.85${\scriptstyle\pm0.16}$ & 99.95${\scriptstyle\pm0.06}$  \\
% CPGNN & 20.38${\scriptstyle\pm1.15}$ & 20.35${\scriptstyle\pm1.41}$ & 19.38${\scriptstyle\pm1.53}$ & 21.32${\scriptstyle\pm1.84}$ & 22.13${\scriptstyle\pm2.79}$ & 24.37${\scriptstyle\pm3.73}$ & 24.93${\scriptstyle\pm4.66}$ & 27.03${\scriptstyle\pm6.61}$ & 28.61${\scriptstyle\pm8.12}$ & 29.7${\scriptstyle\pm9.82}$ & 31.0${\scriptstyle\pm10.87}$  \\
% LP & 9.81${\scriptstyle\pm0.1}$ & 10.1${\scriptstyle\pm0.22}$ & 19.4${\scriptstyle\pm0.22}$ & 31.76${\scriptstyle\pm0.43}$ & 48.44${\scriptstyle\pm0.45}$ & 65.5${\scriptstyle\pm0.74}$ & 81.29${\scriptstyle\pm0.75}$ & 92.91${\scriptstyle\pm0.35}$ & 99.16${\scriptstyle\pm0.11}$ & 99.95${\scriptstyle\pm0.04}$ & 100.0${\scriptstyle\pm0.01}$  \\
% C\&S & 39.44${\scriptstyle\pm3.78}$ & 40.42${\scriptstyle\pm3.5}$ & 42.66${\scriptstyle\pm3.05}$ & 54.18${\scriptstyle\pm1.25}$ & 69.92${\scriptstyle\pm1.71}$ & 86.23${\scriptstyle\pm2.11}$ & 96.55${\scriptstyle\pm0.9}$ & 99.49${\scriptstyle\pm0.17}$ & 99.92${\scriptstyle\pm0.07}$ & 99.92${\scriptstyle\pm0.09}$ & 99.98${\scriptstyle\pm0.03}$  \\
% CLP & 45.7${\scriptstyle\pm0.68}$ & 45.57${\scriptstyle\pm0.45}$ & 49.92${\scriptstyle\pm1.92}$ & 64.1${\scriptstyle\pm1.3}$ & 76.57${\scriptstyle\pm1.54}$ & 84.42${\scriptstyle\pm2.35}$ & 91.1${\scriptstyle\pm0.68}$ & 94.9${\scriptstyle\pm0.79}$ & 97.22${\scriptstyle\pm0.73}$ & 98.82${\scriptstyle\pm0.28}$ & 100.0${\scriptstyle\pm0.0}$  \\
% % \rowcolor{gray!30}
% % CLP\textsuperscript{\dag} & 56.96${\scriptstyle\pm0.95}$ & 45.77${\scriptstyle\pm0.76}$ & 50.94${\scriptstyle\pm0.73}$ & 61.9${\scriptstyle\pm1.87}$ & 83.56${\scriptstyle\pm0.72}$ & 93.57${\scriptstyle\pm0.42}$ & 96.45${\scriptstyle\pm0.36}$ & 97.85${\scriptstyle\pm0.16}$ & 99.52${\scriptstyle\pm0.12}$ & 99.99${\scriptstyle\pm0.01}$ & 100.0${\scriptstyle\pm0.0}$  \\
%         & \multicolumn{11}{c}{\textbf{Train ratio $48\%$}}  \\
% MLP & 45.57${\scriptstyle\pm1.05}$ & 45.44${\scriptstyle\pm0.82}$ & 44.72${\scriptstyle\pm1.27}$ & 46.15${\scriptstyle\pm0.94}$ & 45.26${\scriptstyle\pm1.11}$ & 45.53${\scriptstyle\pm0.92}$ & 45.22${\scriptstyle\pm0.95}$ & 45.0${\scriptstyle\pm0.97}$ & 46.59${\scriptstyle\pm0.69}$ & 46.54${\scriptstyle\pm1.0}$ & 45.46${\scriptstyle\pm0.95}$  \\
% GCN & 27.82${\scriptstyle\pm1.19}$ & 25.2${\scriptstyle\pm1.0}$ & 30.1${\scriptstyle\pm1.34}$ & 45.33${\scriptstyle\pm1.24}$ & 65.23${\scriptstyle\pm1.45}$ & 81.04${\scriptstyle\pm0.69}$ & 93.61${\scriptstyle\pm0.53}$ & 97.68${\scriptstyle\pm0.36}$ & 99.31${\scriptstyle\pm0.18}$ & 99.92${\scriptstyle\pm0.06}$ & 99.99${\scriptstyle\pm0.02}$  \\
% GAT & 30.76${\scriptstyle\pm1.13}$ & 29.32${\scriptstyle\pm1.08}$ & 35.35${\scriptstyle\pm1.32}$ & 49.91${\scriptstyle\pm1.18}$ & 68.12${\scriptstyle\pm1.18}$ & 81.49${\scriptstyle\pm0.99}$ & 92.5${\scriptstyle\pm0.58}$ & 97.12${\scriptstyle\pm0.42}$ & 99.43${\scriptstyle\pm0.16}$ & 99.9${\scriptstyle\pm0.09}$ & 99.96${\scriptstyle\pm0.04}$  \\
% GCN2 & 44.7${\scriptstyle\pm1.24}$ & 43.71${\scriptstyle\pm0.89}$ & 46.14${\scriptstyle\pm1.3}$ & 52.16${\scriptstyle\pm1.18}$ & 58.34${\scriptstyle\pm1.01}$ & 64.33${\scriptstyle\pm0.74}$ & 74.7${\scriptstyle\pm0.7}$ & 83.74${\scriptstyle\pm0.81}$ & 94.55${\scriptstyle\pm0.59}$ & 99.57${\scriptstyle\pm0.13}$ & 99.98${\scriptstyle\pm0.03}$  \\
% SuperGAT & 19.97${\scriptstyle\pm2.18}$ & 20.04${\scriptstyle\pm1.94}$ & 24.99${\scriptstyle\pm1.57}$ & 30.98${\scriptstyle\pm1.73}$ & 41.95${\scriptstyle\pm3.44}$ & 51.1${\scriptstyle\pm4.58}$ & 58.76${\scriptstyle\pm7.67}$ & 65.22${\scriptstyle\pm8.81}$ & 80.24${\scriptstyle\pm6.69}$ & 88.48${\scriptstyle\pm5.19}$ & 94.34${\scriptstyle\pm5.99}$  \\
% GPRGNN & 46.63${\scriptstyle\pm1.16}$ & 44.69${\scriptstyle\pm0.93}$ & 46.06${\scriptstyle\pm1.49}$ & 53.86${\scriptstyle\pm1.17}$ & 67.18${\scriptstyle\pm1.45}$ & 80.9${\scriptstyle\pm2.42}$ & 89.05${\scriptstyle\pm2.94}$ & 92.69${\scriptstyle\pm2.06}$ & 98.2${\scriptstyle\pm0.48}$ & 99.79${\scriptstyle\pm0.08}$ & 99.99${\scriptstyle\pm0.02}$  \\
% FAGCN & 47.18${\scriptstyle\pm1.06}$ & 45.83${\scriptstyle\pm1.02}$ & 46.26${\scriptstyle\pm1.2}$ & 53.21${\scriptstyle\pm1.85}$ & 65.2${\scriptstyle\pm4.43}$ & 74.49${\scriptstyle\pm7.79}$ & 85.41${\scriptstyle\pm5.59}$ & 92.42${\scriptstyle\pm4.16}$ & 98.16${\scriptstyle\pm1.37}$ & 99.39${\scriptstyle\pm0.64}$ & 99.86${\scriptstyle\pm0.1}$  \\
% H2GCN & 51.64${\scriptstyle\pm0.94}$ & 44.42${\scriptstyle\pm0.85}$ & 49.33${\scriptstyle\pm1.37}$ & 64.52${\scriptstyle\pm1.24}$ & 78.95${\scriptstyle\pm2.51}$ & 91.56${\scriptstyle\pm1.41}$ & 97.5${\scriptstyle\pm0.7}$ & 99.04${\scriptstyle\pm0.28}$ & 99.75${\scriptstyle\pm0.12}$ & 99.96${\scriptstyle\pm0.05}$ & 99.98${\scriptstyle\pm0.04}$  \\
% CPGNN & 19.79${\scriptstyle\pm2.1}$ & 18.51${\scriptstyle\pm1.79}$ & 19.36${\scriptstyle\pm1.22}$ & 22.39${\scriptstyle\pm1.64}$ & 19.39${\scriptstyle\pm3.2}$ & 24.3${\scriptstyle\pm4.38}$ & 24.75${\scriptstyle\pm5.64}$ & 25.94${\scriptstyle\pm7.89}$ & 31.11${\scriptstyle\pm10.13}$ & 30.76${\scriptstyle\pm11.94}$ & 32.64${\scriptstyle\pm12.37}$  \\
% LP & 9.54${\scriptstyle\pm0.63}$ & 9.57${\scriptstyle\pm0.75}$ & 31.15${\scriptstyle\pm0.42}$ & 56.28${\scriptstyle\pm1.2}$ & 78.28${\scriptstyle\pm1.07}$ & 91.86${\scriptstyle\pm0.57}$ & 97.9${\scriptstyle\pm0.34}$ & 99.5${\scriptstyle\pm0.2}$ & 99.91${\scriptstyle\pm0.05}$ & 99.97${\scriptstyle\pm0.04}$ & 100.0${\scriptstyle\pm0.0}$  \\
% C\&S & 37.76${\scriptstyle\pm5.53}$ & 39.52${\scriptstyle\pm2.64}$ & 56.82${\scriptstyle\pm1.31}$ & 75.84${\scriptstyle\pm1.2}$ & 89.67${\scriptstyle\pm1.15}$ & 96.9${\scriptstyle\pm0.63}$ & 99.31${\scriptstyle\pm0.16}$ & 99.87${\scriptstyle\pm0.07}$ & 99.96${\scriptstyle\pm0.04}$ & 99.97${\scriptstyle\pm0.04}$ & 100.0${\scriptstyle\pm0.0}$  \\
% CLP & 53.45${\scriptstyle\pm1.36}$ & 45.54${\scriptstyle\pm0.53}$ & 48.34${\scriptstyle\pm0.91}$ & 59.74${\scriptstyle\pm2.75}$ & 71.99${\scriptstyle\pm2.72}$ & 81.61${\scriptstyle\pm3.8}$ & 88.82${\scriptstyle\pm2.58}$ & 93.76${\scriptstyle\pm1.69}$ & 96.24${\scriptstyle\pm1.28}$ & 98.57${\scriptstyle\pm0.65}$ & 99.97${\scriptstyle\pm0.03}$  \\
% % \rowcolor{gray!30}
% % CLP\textsuperscript{\dag} & 71.51${\scriptstyle\pm0.91}$ & 46.09${\scriptstyle\pm0.97}$ & 60.5${\scriptstyle\pm1.25}$ & 74.56${\scriptstyle\pm1.42}$ & 90.17${\scriptstyle\pm0.62}$ & 97.27${\scriptstyle\pm0.28}$ & 99.13${\scriptstyle\pm0.18}$ & 99.38${\scriptstyle\pm0.18}$ & 99.64${\scriptstyle\pm0.15}$ & 99.99${\scriptstyle\pm0.02}$ & 100.0${\scriptstyle\pm0.0}$  \\
% \hline
% \end{tabular}
% }
% \end{table*}

% \begin{table*}
% \caption{Node classification results of Syn-Products-1 dataset. 
% % \textsuperscript{\dag} means utilise spectral features.
% }
% % \vspace{-3mm}
% \label{table:NC_experimental_results_p_syn_self_005}
% % \small
% \centering
% \resizebox{.7\textwidth}{!}{
% \begin{tabular}{l ccccccccccc}
% \hline
% $h$     & 0.0 & 0.1 & 0.2 & 0.3 & 0.4 & 0.5 & 0.6 & 0.7 & 0.8 & 0.9 & 1.0\\
%         & \multicolumn{11}{c}{\textbf{Train ratio $5\%$}}  \\
% MLP & 57.61${\scriptstyle\pm1.31}$ & 56.88${\scriptstyle\pm0.98}$ & 56.25${\scriptstyle\pm0.91}$ & 57.72${\scriptstyle\pm0.82}$ & 56.87${\scriptstyle\pm0.84}$ & 57.07${\scriptstyle\pm0.87}$ & 56.66${\scriptstyle\pm0.73}$ & 56.69${\scriptstyle\pm0.74}$ & 56.98${\scriptstyle\pm0.93}$ & 57.57${\scriptstyle\pm1.0}$ & 58.09${\scriptstyle\pm1.0}$  \\
% GCN & 23.24${\scriptstyle\pm0.6}$ & 26.65${\scriptstyle\pm0.62}$ & 32.53${\scriptstyle\pm0.94}$ & 41.14${\scriptstyle\pm0.85}$ & 51.07${\scriptstyle\pm0.77}$ & 62.58${\scriptstyle\pm0.77}$ & 73.4${\scriptstyle\pm0.8}$ & 83.64${\scriptstyle\pm0.45}$ & 90.26${\scriptstyle\pm0.39}$ & 95.31${\scriptstyle\pm0.16}$ & 98.05${\scriptstyle\pm0.28}$  \\
% GAT & 9.87${\scriptstyle\pm0.09}$ & 10.66${\scriptstyle\pm2.93}$ & 9.84${\scriptstyle\pm0.05}$ & 12.68${\scriptstyle\pm8.3}$ & 9.86${\scriptstyle\pm0.08}$ & 24.53${\scriptstyle\pm22.49}$ & 11.0${\scriptstyle\pm1.71}$ & 22.76${\scriptstyle\pm25.86}$ & 14.31${\scriptstyle\pm17.91}$ & 11.91${\scriptstyle\pm6.13}$ & 22.76${\scriptstyle\pm26.0}$  \\
% GCN2 & 43.28${\scriptstyle\pm6.45}$ & 43.9${\scriptstyle\pm3.98}$ & 44.91${\scriptstyle\pm1.64}$ & 51.75${\scriptstyle\pm1.59}$ & 57.76${\scriptstyle\pm1.36}$ & 66.07${\scriptstyle\pm1.22}$ & 74.61${\scriptstyle\pm1.0}$ & 85.01${\scriptstyle\pm0.73}$ & 92.46${\scriptstyle\pm0.73}$ & 97.48${\scriptstyle\pm0.2}$ & 99.43${\scriptstyle\pm0.16}$  \\
% SuperGAT & 9.92${\scriptstyle\pm0.09}$ & 10.07${\scriptstyle\pm0.43}$ & 9.98${\scriptstyle\pm0.41}$ & 9.88${\scriptstyle\pm0.09}$ & 10.71${\scriptstyle\pm3.6}$ & 10.07${\scriptstyle\pm0.44}$ & 13.83${\scriptstyle\pm10.39}$ & 10.59${\scriptstyle\pm1.46}$ & 17.01${\scriptstyle\pm16.28}$ & 13.09${\scriptstyle\pm10.08}$ & 13.65${\scriptstyle\pm13.74}$  \\
% GPRGNN & 56.1${\scriptstyle\pm1.17}$ & 55.38${\scriptstyle\pm1.14}$ & 55.39${\scriptstyle\pm1.37}$ & 58.44${\scriptstyle\pm1.03}$ & 61.36${\scriptstyle\pm0.8}$ & 67.92${\scriptstyle\pm1.22}$ & 77.53${\scriptstyle\pm0.86}$ & 88.33${\scriptstyle\pm0.6}$ & 94.1${\scriptstyle\pm0.54}$ & 97.84${\scriptstyle\pm0.18}$ & 99.5${\scriptstyle\pm0.16}$  \\
% FAGCN & 51.53${\scriptstyle\pm1.62}$ & 51.03${\scriptstyle\pm1.2}$ & 50.35${\scriptstyle\pm1.21}$ & 53.85${\scriptstyle\pm0.9}$ & 57.46${\scriptstyle\pm1.08}$ & 62.68${\scriptstyle\pm1.99}$ & 68.22${\scriptstyle\pm3.02}$ & 76.4${\scriptstyle\pm0.99}$ & 82.04${\scriptstyle\pm1.99}$ & 88.59${\scriptstyle\pm0.71}$ & 92.3${\scriptstyle\pm1.86}$  \\
% H2GCN & 55.89${\scriptstyle\pm1.1}$ & 54.63${\scriptstyle\pm1.31}$ & 54.2${\scriptstyle\pm1.15}$ & 57.2${\scriptstyle\pm0.71}$ & 59.61${\scriptstyle\pm1.08}$ & 66.49${\scriptstyle\pm1.3}$ & 76.12${\scriptstyle\pm1.25}$ & 86.2${\scriptstyle\pm0.92}$ & 92.83${\scriptstyle\pm0.37}$ & 97.11${\scriptstyle\pm0.19}$ & 99.03${\scriptstyle\pm0.18}$  \\
% % CPGNN & & & & & & & & & & &  \\
% LP & 9.5${\scriptstyle\pm0.66}$ & 10.27${\scriptstyle\pm0.22}$ & 12.86${\scriptstyle\pm0.39}$ & 16.98${\scriptstyle\pm0.25}$ & 23.38${\scriptstyle\pm0.66}$ & 32.32${\scriptstyle\pm0.83}$ & 46.25${\scriptstyle\pm0.7}$ & 65.99${\scriptstyle\pm1.03}$ & 82.54${\scriptstyle\pm0.74}$ & 94.41${\scriptstyle\pm0.28}$ & 99.37${\scriptstyle\pm0.03}$  \\
% C\&S & 57.54${\scriptstyle\pm1.24}$ & 56.7${\scriptstyle\pm1.26}$ & 56.27${\scriptstyle\pm1.54}$ & 59.08${\scriptstyle\pm1.16}$ & 60.68${\scriptstyle\pm1.69}$ & 65.29${\scriptstyle\pm2.56}$ & 70.86${\scriptstyle\pm4.47}$ & 79.53${\scriptstyle\pm5.94}$ & 86.87${\scriptstyle\pm5.03}$ & 96.98${\scriptstyle\pm2.09}$ & 99.61${\scriptstyle\pm0.15}$  \\
% CLP & 57.78${\scriptstyle\pm1.29}$ & 55.99${\scriptstyle\pm1.19}$ & 56.58${\scriptstyle\pm1.25}$ & 59.42${\scriptstyle\pm1.53}$ & 61.07${\scriptstyle\pm1.24}$ & 65.34${\scriptstyle\pm1.49}$ & 70.11${\scriptstyle\pm1.77}$ & 77.41${\scriptstyle\pm1.11}$ & 83.98${\scriptstyle\pm1.02}$ & 91.44${\scriptstyle\pm1.09}$ & 99.32${\scriptstyle\pm0.08}$  \\
% % \rowcolor{gray!30}
% % CLP\textsuperscript{\dag} & 58.11${\scriptstyle\pm1.28}$ & 57.36${\scriptstyle\pm0.98}$ & 57.98${\scriptstyle\pm0.9}$ & 59.0${\scriptstyle\pm0.98}$ & 63.5${\scriptstyle\pm0.88}$ & 69.66${\scriptstyle\pm1.19}$ & 76.15${\scriptstyle\pm1.23}$ & 83.75${\scriptstyle\pm0.63}$ & 90.18${\scriptstyle\pm0.71}$ & 95.6${\scriptstyle\pm0.39}$ & 99.29${\scriptstyle\pm0.05}$  \\
%         & \multicolumn{11}{c}{\textbf{Train ratio $10\%$}}  \\
% MLP & 62.66${\scriptstyle\pm0.75}$ & 61.41${\scriptstyle\pm0.53}$ & 61.35${\scriptstyle\pm0.39}$ & 61.98${\scriptstyle\pm0.75}$ & 61.32${\scriptstyle\pm0.41}$ & 61.78${\scriptstyle\pm0.55}$ & 61.58${\scriptstyle\pm0.65}$ & 61.3${\scriptstyle\pm0.65}$ & 61.85${\scriptstyle\pm0.63}$ & 62.18${\scriptstyle\pm0.61}$ & 62.23${\scriptstyle\pm0.47}$  \\
% GCN & 25.6${\scriptstyle\pm0.75}$ & 29.21${\scriptstyle\pm0.64}$ & 35.62${\scriptstyle\pm0.81}$ & 44.14${\scriptstyle\pm0.53}$ & 54.55${\scriptstyle\pm0.66}$ & 66.0${\scriptstyle\pm0.44}$ & 76.12${\scriptstyle\pm0.51}$ & 85.39${\scriptstyle\pm0.37}$ & 91.35${\scriptstyle\pm0.26}$ & 95.69${\scriptstyle\pm0.23}$ & 98.49${\scriptstyle\pm0.17}$  \\
% GAT & 11.16${\scriptstyle\pm4.26}$ & 9.81${\scriptstyle\pm0.31}$ & 11.03${\scriptstyle\pm5.3}$ & 11.33${\scriptstyle\pm6.53}$ & 12.67${\scriptstyle\pm10.11}$ & 24.72${\scriptstyle\pm24.55}$ & 10.58${\scriptstyle\pm1.44}$ & 12.16${\scriptstyle\pm3.63}$ & 14.83${\scriptstyle\pm18.02}$ & 11.46${\scriptstyle\pm2.98}$ & 17.78${\scriptstyle\pm19.39}$  \\
% GCN2 & 55.54${\scriptstyle\pm4.48}$ & 55.36${\scriptstyle\pm1.86}$ & 53.42${\scriptstyle\pm2.95}$ & 54.25${\scriptstyle\pm1.63}$ & 60.91${\scriptstyle\pm1.26}$ & 67.91${\scriptstyle\pm1.17}$ & 77.06${\scriptstyle\pm0.62}$ & 86.77${\scriptstyle\pm0.48}$ & 93.48${\scriptstyle\pm0.34}$ & 97.63${\scriptstyle\pm0.18}$ & 99.49${\scriptstyle\pm0.12}$  \\
% SuperGAT & 9.78${\scriptstyle\pm0.2}$ & 9.89${\scriptstyle\pm0.29}$ & 9.96${\scriptstyle\pm0.29}$ & 9.97${\scriptstyle\pm0.54}$ & 11.0${\scriptstyle\pm3.67}$ & 11.1${\scriptstyle\pm3.65}$ & 12.14${\scriptstyle\pm8.21}$ & 13.58${\scriptstyle\pm11.93}$ & 12.09${\scriptstyle\pm9.82}$ & 13.87${\scriptstyle\pm13.95}$ & 17.96${\scriptstyle\pm20.95}$  \\
% GPRGNN & 60.96${\scriptstyle\pm0.84}$ & 59.61${\scriptstyle\pm0.87}$ & 59.5${\scriptstyle\pm0.87}$ & 61.77${\scriptstyle\pm0.88}$ & 64.99${\scriptstyle\pm1.34}$ & 70.5${\scriptstyle\pm0.92}$ & 78.81${\scriptstyle\pm0.89}$ & 88.63${\scriptstyle\pm0.55}$ & 94.49${\scriptstyle\pm0.35}$ & 97.93${\scriptstyle\pm0.2}$ & 99.59${\scriptstyle\pm0.09}$  \\
% FAGCN & 56.26${\scriptstyle\pm0.58}$ & 55.36${\scriptstyle\pm0.99}$ & 54.95${\scriptstyle\pm0.8}$ & 57.43${\scriptstyle\pm1.1}$ & 61.32${\scriptstyle\pm1.33}$ & 66.97${\scriptstyle\pm0.9}$ & 73.26${\scriptstyle\pm0.62}$ & 80.57${\scriptstyle\pm0.58}$ & 85.32${\scriptstyle\pm1.47}$ & 89.78${\scriptstyle\pm1.94}$ & 94.14${\scriptstyle\pm0.96}$  \\
% H2GCN & 62.14${\scriptstyle\pm0.91}$ & 60.34${\scriptstyle\pm0.87}$ & 60.61${\scriptstyle\pm0.8}$ & 62.57${\scriptstyle\pm0.92}$ & 66.07${\scriptstyle\pm0.7}$ & 73.59${\scriptstyle\pm1.21}$ & 81.59${\scriptstyle\pm0.7}$ & 89.58${\scriptstyle\pm0.39}$ & 94.28${\scriptstyle\pm0.35}$ & 97.56${\scriptstyle\pm0.2}$ & 99.31${\scriptstyle\pm0.12}$  \\
% % CPGNN & & & & & & & & & & &  \\
% LP & 9.52${\scriptstyle\pm0.85}$ & 10.02${\scriptstyle\pm0.33}$ & 14.78${\scriptstyle\pm0.39}$ & 20.58${\scriptstyle\pm0.53}$ & 29.73${\scriptstyle\pm0.58}$ & 40.8${\scriptstyle\pm0.72}$ & 55.19${\scriptstyle\pm0.55}$ & 73.27${\scriptstyle\pm0.65}$ & 86.07${\scriptstyle\pm0.43}$ & 95.59${\scriptstyle\pm0.22}$ & 99.39${\scriptstyle\pm0.04}$  \\
% C\&S & 62.45${\scriptstyle\pm0.83}$ & 61.32${\scriptstyle\pm0.61}$ & 61.43${\scriptstyle\pm0.82}$ & 63.01${\scriptstyle\pm0.74}$ & 65.01${\scriptstyle\pm1.66}$ & 69.31${\scriptstyle\pm2.34}$ & 75.28${\scriptstyle\pm3.66}$ & 85.29${\scriptstyle\pm4.59}$ & 91.26${\scriptstyle\pm2.53}$ & 97.17${\scriptstyle\pm0.75}$ & 99.77${\scriptstyle\pm0.03}$  \\
% CLP & 62.82${\scriptstyle\pm0.72}$ & 60.8${\scriptstyle\pm1.12}$ & 61.54${\scriptstyle\pm1.14}$ & 63.58${\scriptstyle\pm0.72}$ & 65.83${\scriptstyle\pm0.58}$ & 70.91${\scriptstyle\pm0.84}$ & 76.62${\scriptstyle\pm0.58}$ & 82.76${\scriptstyle\pm0.97}$ & 87.86${\scriptstyle\pm0.34}$ & 93.31${\scriptstyle\pm0.44}$ & 99.3${\scriptstyle\pm0.09}$  \\
% % \rowcolor{gray!30}
% % CLP\textsuperscript{\dag} & 63.55${\scriptstyle\pm0.69}$ & 62.81${\scriptstyle\pm0.66}$ & 64.11${\scriptstyle\pm0.54}$ & 63.52${\scriptstyle\pm1.23}$ & 69.69${\scriptstyle\pm0.62}$ & 75.79${\scriptstyle\pm0.69}$ & 82.08${\scriptstyle\pm0.43}$ & 88.49${\scriptstyle\pm0.38}$ & 93.26${\scriptstyle\pm0.24}$ & 96.95${\scriptstyle\pm0.19}$ & 99.33${\scriptstyle\pm0.05}$  \\
%         & \multicolumn{11}{c}{\textbf{Train ratio $48\%$}}  \\
% MLP & 72.53${\scriptstyle\pm1.05}$ & 71.45${\scriptstyle\pm0.85}$ & 71.07${\scriptstyle\pm1.26}$ & 72.33${\scriptstyle\pm0.7}$ & 70.82${\scriptstyle\pm0.61}$ & 71.58${\scriptstyle\pm1.12}$ & 71.66${\scriptstyle\pm0.82}$ & 71.68${\scriptstyle\pm1.2}$ & 71.33${\scriptstyle\pm0.75}$ & 72.29${\scriptstyle\pm1.12}$ & 72.19${\scriptstyle\pm0.99}$  \\
% GCN & 31.14${\scriptstyle\pm0.7}$ & 34.99${\scriptstyle\pm0.99}$ & 42.47${\scriptstyle\pm0.61}$ & 52.53${\scriptstyle\pm0.81}$ & 61.6${\scriptstyle\pm0.7}$ & 71.52${\scriptstyle\pm0.89}$ & 81.24${\scriptstyle\pm0.67}$ & 88.61${\scriptstyle\pm0.78}$ & 93.13${\scriptstyle\pm0.43}$ & 96.91${\scriptstyle\pm0.37}$ & 99.1${\scriptstyle\pm0.23}$  \\
% GAT & 9.29${\scriptstyle\pm0.38}$ & 10.76${\scriptstyle\pm5.96}$ & 11.03${\scriptstyle\pm7.0}$ & 9.54${\scriptstyle\pm0.49}$ & 9.4${\scriptstyle\pm0.66}$ & 18.45${\scriptstyle\pm21.41}$ & 10.32${\scriptstyle\pm1.64}$ & 18.67${\scriptstyle\pm23.86}$ & 9.4${\scriptstyle\pm1.13}$ & 11.1${\scriptstyle\pm2.59}$ & 27.54${\scriptstyle\pm30.79}$  \\
% GCN2 & 61.04${\scriptstyle\pm1.68}$ & 60.87${\scriptstyle\pm1.09}$ & 60.26${\scriptstyle\pm1.72}$ & 60.54${\scriptstyle\pm0.87}$ & 64.03${\scriptstyle\pm1.02}$ & 70.14${\scriptstyle\pm1.13}$ & 79.77${\scriptstyle\pm1.12}$ & 88.07${\scriptstyle\pm0.92}$ & 94.3${\scriptstyle\pm0.44}$ & 98.02${\scriptstyle\pm0.26}$ & 99.7${\scriptstyle\pm0.11}$  \\
% SuperGAT & 9.66${\scriptstyle\pm0.78}$ & 9.62${\scriptstyle\pm0.55}$ & 9.46${\scriptstyle\pm0.44}$ & 9.41${\scriptstyle\pm0.5}$ & 10.87${\scriptstyle\pm6.44}$ & 12.53${\scriptstyle\pm5.65}$ & 9.72${\scriptstyle\pm0.77}$ & 17.77${\scriptstyle\pm19.56}$ & 12.61${\scriptstyle\pm13.24}$ & 21.92${\scriptstyle\pm25.74}$ & 19.8${\scriptstyle\pm25.07}$  \\
% GPRGNN & 65.4${\scriptstyle\pm1.6}$ & 63.86${\scriptstyle\pm0.79}$ & 63.83${\scriptstyle\pm1.25}$ & 67.14${\scriptstyle\pm1.1}$ & 69.91${\scriptstyle\pm0.65}$ & 72.99${\scriptstyle\pm1.52}$ & 80.47${\scriptstyle\pm0.97}$ & 89.91${\scriptstyle\pm0.88}$ & 94.55${\scriptstyle\pm0.56}$ & 98.16${\scriptstyle\pm0.29}$ & 99.77${\scriptstyle\pm0.08}$  \\
% FAGCN & 61.58${\scriptstyle\pm0.99}$ & 61.02${\scriptstyle\pm0.86}$ & 61.06${\scriptstyle\pm1.27}$ & 63.68${\scriptstyle\pm0.95}$ & 66.79${\scriptstyle\pm0.81}$ & 72.43${\scriptstyle\pm1.01}$ & 79.22${\scriptstyle\pm0.87}$ & 84.87${\scriptstyle\pm1.42}$ & 90.12${\scriptstyle\pm0.7}$ & 94.05${\scriptstyle\pm0.74}$ & 96.48${\scriptstyle\pm0.67}$  \\
% H2GCN & 72.87${\scriptstyle\pm0.89}$ & 70.66${\scriptstyle\pm0.77}$ & 70.72${\scriptstyle\pm1.27}$ & 74.6${\scriptstyle\pm0.68}$ & 78.71${\scriptstyle\pm0.65}$ & 84.89${\scriptstyle\pm0.81}$ & 90.17${\scriptstyle\pm0.71}$ & 93.74${\scriptstyle\pm0.72}$ & 96.24${\scriptstyle\pm0.52}$ & 98.25${\scriptstyle\pm0.21}$ & 99.67${\scriptstyle\pm0.08}$  \\
% % CPGNN & & & & & & & & & & &  \\
% LP & 9.3${\scriptstyle\pm0.45}$ & 10.51${\scriptstyle\pm0.73}$ & 21.68${\scriptstyle\pm0.76}$ & 33.88${\scriptstyle\pm1.03}$ & 48.05${\scriptstyle\pm1.02}$ & 62.21${\scriptstyle\pm0.72}$ & 75.41${\scriptstyle\pm0.85}$ & 86.86${\scriptstyle\pm0.5}$ & 93.12${\scriptstyle\pm0.53}$ & 97.65${\scriptstyle\pm0.31}$ & 99.38${\scriptstyle\pm0.15}$  \\
% C\&S & 72.08${\scriptstyle\pm0.77}$ & 71.4${\scriptstyle\pm0.74}$ & 72.04${\scriptstyle\pm1.31}$ & 74.74${\scriptstyle\pm0.73}$ & 76.25${\scriptstyle\pm1.23}$ & 81.46${\scriptstyle\pm1.06}$ & 87.93${\scriptstyle\pm1.07}$ & 93.43${\scriptstyle\pm0.57}$ & 96.78${\scriptstyle\pm0.31}$ & 98.84${\scriptstyle\pm0.19}$ & 99.9${\scriptstyle\pm0.05}$  \\
% CLP & 72.29${\scriptstyle\pm0.94}$ & 70.06${\scriptstyle\pm2.12}$ & 71.28${\scriptstyle\pm1.92}$ & 74.89${\scriptstyle\pm1.11}$ & 76.71${\scriptstyle\pm0.75}$ & 81.37${\scriptstyle\pm0.88}$ & 86.07${\scriptstyle\pm0.74}$ & 90.49${\scriptstyle\pm0.53}$ & 93.45${\scriptstyle\pm0.29}$ & 96.63${\scriptstyle\pm0.46}$ & 99.35${\scriptstyle\pm0.15}$  \\
% % \rowcolor{gray!30}
% % CLP\textsuperscript{\dag} & 73.56${\scriptstyle\pm0.99}$ & 73.18${\scriptstyle\pm0.66}$ & 74.79${\scriptstyle\pm1.29}$ & 74.83${\scriptstyle\pm0.79}$ & 80.61${\scriptstyle\pm0.82}$ & 84.58${\scriptstyle\pm0.75}$ & 89.58${\scriptstyle\pm0.67}$ & 93.5${\scriptstyle\pm0.54}$ & 96.18${\scriptstyle\pm0.3}$ & 98.44${\scriptstyle\pm0.16}$ & 99.38${\scriptstyle\pm0.16}$  \\
% \hline
% \end{tabular}
% }
% \end{table*}

% \begin{table*}
% \caption{Node classification results of Syn-Products-2 dataset. 
% % \textsuperscript{\dag} means utilise spectral features.
% }
% % \vspace{-3mm}
% \label{table:NC_experimental_results_p_syn_self_010}
% % \small
% \centering
% \resizebox{.7\textwidth}{!}{
% \begin{tabular}{l ccccccccccc}
% \hline
% $h$     & 0.0 & 0.1 & 0.2 & 0.3 & 0.4 & 0.5 & 0.6 & 0.7 & 0.8 & 0.9 & 1.0\\
%         & \multicolumn{11}{c}{\textbf{Train ratio $5\%$}}  \\
% MLP & 56.43${\scriptstyle\pm0.94}$ & 57.1${\scriptstyle\pm0.83}$ & 57.0${\scriptstyle\pm0.89}$ & 58.11${\scriptstyle\pm1.01}$ & 56.53${\scriptstyle\pm1.06}$ & 57.64${\scriptstyle\pm1.22}$ & 56.38${\scriptstyle\pm0.88}$ & 57.42${\scriptstyle\pm1.08}$ & 56.63${\scriptstyle\pm0.93}$ & 56.84${\scriptstyle\pm0.81}$ & 56.74${\scriptstyle\pm1.07}$  \\
% GCN & 24.01${\scriptstyle\pm0.65}$ & 26.17${\scriptstyle\pm0.74}$ & 35.05${\scriptstyle\pm0.63}$ & 48.67${\scriptstyle\pm0.69}$ & 64.39${\scriptstyle\pm0.74}$ & 79.48${\scriptstyle\pm0.64}$ & 90.25${\scriptstyle\pm0.44}$ & 96.28${\scriptstyle\pm0.23}$ & 98.67${\scriptstyle\pm0.22}$ & 99.6${\scriptstyle\pm0.09}$ & 99.83${\scriptstyle\pm0.08}$  \\
% GAT & 10.24${\scriptstyle\pm1.27}$ & 10.04${\scriptstyle\pm0.97}$ & 9.84${\scriptstyle\pm0.14}$ & 10.2${\scriptstyle\pm0.61}$ & 9.87${\scriptstyle\pm0.05}$ & 30.41${\scriptstyle\pm30.98}$ & 14.14${\scriptstyle\pm17.58}$ & 10.23${\scriptstyle\pm0.93}$ & 14.62${\scriptstyle\pm19.36}$ & 16.55${\scriptstyle\pm19.28}$ & 10.29${\scriptstyle\pm0.55}$  \\
% GCN2 & 49.18${\scriptstyle\pm5.17}$ & 47.64${\scriptstyle\pm2.73}$ & 53.01${\scriptstyle\pm1.04}$ & 59.26${\scriptstyle\pm1.19}$ & 65.57${\scriptstyle\pm0.97}$ & 74.99${\scriptstyle\pm1.35}$ & 84.68${\scriptstyle\pm1.15}$ & 92.91${\scriptstyle\pm0.55}$ & 97.66${\scriptstyle\pm0.17}$ & 99.48${\scriptstyle\pm0.12}$ & 99.82${\scriptstyle\pm0.15}$  \\
% SuperGAT & 9.9${\scriptstyle\pm0.08}$ & 9.98${\scriptstyle\pm0.37}$ & 9.88${\scriptstyle\pm0.12}$ & 10.14${\scriptstyle\pm0.57}$ & 9.94${\scriptstyle\pm0.26}$ & 10.17${\scriptstyle\pm0.72}$ & 11.31${\scriptstyle\pm2.31}$ & 10.25${\scriptstyle\pm0.83}$ & 11.0${\scriptstyle\pm2.29}$ & 16.84${\scriptstyle\pm19.0}$ & 13.29${\scriptstyle\pm11.02}$  \\
% GPRGNN & 56.52${\scriptstyle\pm1.0}$ & 55.2${\scriptstyle\pm1.11}$ & 56.28${\scriptstyle\pm0.92}$ & 62.35${\scriptstyle\pm0.92}$ & 72.13${\scriptstyle\pm1.47}$ & 84.42${\scriptstyle\pm1.69}$ & 93.19${\scriptstyle\pm0.85}$ & 97.5${\scriptstyle\pm0.44}$ & 99.13${\scriptstyle\pm0.25}$ & 99.79${\scriptstyle\pm0.09}$ & 99.9${\scriptstyle\pm0.11}$  \\
% FAGCN & 50.86${\scriptstyle\pm1.0}$ & 51.7${\scriptstyle\pm0.72}$ & 52.61${\scriptstyle\pm1.05}$ & 58.41${\scriptstyle\pm0.79}$ & 63.91${\scriptstyle\pm0.71}$ & 71.86${\scriptstyle\pm1.0}$ & 79.48${\scriptstyle\pm2.65}$ & 86.12${\scriptstyle\pm2.42}$ & 91.04${\scriptstyle\pm2.82}$ & 95.06${\scriptstyle\pm0.6}$ & 97.12${\scriptstyle\pm0.96}$  \\
% H2GCN & 55.06${\scriptstyle\pm1.36}$ & 54.3${\scriptstyle\pm0.98}$ & 55.59${\scriptstyle\pm0.88}$ & 60.28${\scriptstyle\pm1.0}$ & 68.14${\scriptstyle\pm1.61}$ & 82.13${\scriptstyle\pm1.28}$ & 91.56${\scriptstyle\pm1.12}$ & 97.15${\scriptstyle\pm0.32}$ & 99.03${\scriptstyle\pm0.26}$ & 99.69${\scriptstyle\pm0.1}$ & 99.86${\scriptstyle\pm0.11}$  \\
% % CPGNN & & & & & & & & & & &  \\
% LP & 9.89${\scriptstyle\pm0.05}$ & 9.91${\scriptstyle\pm0.28}$ & 15.18${\scriptstyle\pm0.4}$ & 22.6${\scriptstyle\pm0.35}$ & 33.11${\scriptstyle\pm0.94}$ & 47.99${\scriptstyle\pm1.06}$ & 67.64${\scriptstyle\pm1.03}$ & 83.85${\scriptstyle\pm0.85}$ & 93.47${\scriptstyle\pm0.47}$ & 98.84${\scriptstyle\pm0.15}$ & 100.0${\scriptstyle\pm0.01}$  \\
% C\&S & 56.42${\scriptstyle\pm1.06}$ & 56.25${\scriptstyle\pm2.46}$ & 57.16${\scriptstyle\pm1.38}$ & 60.02${\scriptstyle\pm1.61}$ & 61.16${\scriptstyle\pm2.58}$ & 69.94${\scriptstyle\pm5.11}$ & 72.38${\scriptstyle\pm7.54}$ & 84.01${\scriptstyle\pm8.42}$ & 92.8${\scriptstyle\pm5.75}$ & 98.99${\scriptstyle\pm1.24}$ & 99.98${\scriptstyle\pm0.04}$  \\
% CLP & 56.69${\scriptstyle\pm1.35}$ & 56.38${\scriptstyle\pm1.23}$ & 57.49${\scriptstyle\pm1.69}$ & 61.78${\scriptstyle\pm1.47}$ & 64.74${\scriptstyle\pm1.77}$ & 70.12${\scriptstyle\pm1.68}$ & 75.8${\scriptstyle\pm1.51}$ & 80.77${\scriptstyle\pm2.41}$ & 85.73${\scriptstyle\pm2.4}$ & 91.99${\scriptstyle\pm1.02}$ & 99.95${\scriptstyle\pm0.08}$  \\
% % \rowcolor{gray!30}
% % CLP\textsuperscript{\dag} & 56.7${\scriptstyle\pm1.02}$ & 56.94${\scriptstyle\pm0.61}$ & 58.49${\scriptstyle\pm1.1}$ & 62.53${\scriptstyle\pm0.98}$ & 67.09${\scriptstyle\pm1.04}$ & 73.8${\scriptstyle\pm0.87}$ & 80.31${\scriptstyle\pm0.68}$ & 86.17${\scriptstyle\pm0.86}$ & 91.98${\scriptstyle\pm0.59}$ & 96.1${\scriptstyle\pm0.56}$ & 99.9${\scriptstyle\pm0.06}$  \\
%         & \multicolumn{11}{c}{\textbf{Train ratio $10\%$}}  \\
% MLP & 62.05${\scriptstyle\pm0.74}$ & 61.9${\scriptstyle\pm0.74}$ & 61.51${\scriptstyle\pm0.75}$ & 62.15${\scriptstyle\pm1.0}$ & 61.39${\scriptstyle\pm0.88}$ & 62.34${\scriptstyle\pm0.65}$ & 61.55${\scriptstyle\pm0.77}$ & 61.73${\scriptstyle\pm0.99}$ & 61.74${\scriptstyle\pm1.1}$ & 61.7${\scriptstyle\pm0.73}$ & 61.7${\scriptstyle\pm0.59}$  \\
% GCN & 26.51${\scriptstyle\pm0.62}$ & 29.29${\scriptstyle\pm0.63}$ & 38.5${\scriptstyle\pm0.76}$ & 52.26${\scriptstyle\pm0.59}$ & 67.8${\scriptstyle\pm0.63}$ & 81.75${\scriptstyle\pm0.48}$ & 91.53${\scriptstyle\pm0.35}$ & 96.65${\scriptstyle\pm0.22}$ & 98.92${\scriptstyle\pm0.12}$ & 99.63${\scriptstyle\pm0.1}$ & 99.84${\scriptstyle\pm0.11}$  \\
% GAT & 10.81${\scriptstyle\pm3.35}$ & 10.76${\scriptstyle\pm4.04}$ & 11.72${\scriptstyle\pm6.16}$ & 10.07${\scriptstyle\pm1.11}$ & 13.02${\scriptstyle\pm13.37}$ & 15.42${\scriptstyle\pm17.64}$ & 14.1${\scriptstyle\pm18.28}$ & 10.8${\scriptstyle\pm2.01}$ & 10.54${\scriptstyle\pm1.7}$ & 12.48${\scriptstyle\pm3.35}$ & 19.84${\scriptstyle\pm26.83}$  \\
% GCN2 & 57.76${\scriptstyle\pm0.97}$ & 55.64${\scriptstyle\pm2.51}$ & 55.97${\scriptstyle\pm1.16}$ & 62.39${\scriptstyle\pm0.9}$ & 68.55${\scriptstyle\pm0.9}$ & 78.02${\scriptstyle\pm0.84}$ & 86.34${\scriptstyle\pm0.87}$ & 93.89${\scriptstyle\pm0.37}$ & 98.0${\scriptstyle\pm0.2}$ & 99.54${\scriptstyle\pm0.11}$ & 99.88${\scriptstyle\pm0.06}$  \\
% SuperGAT & 9.93${\scriptstyle\pm0.22}$ & 9.85${\scriptstyle\pm0.3}$ & 10.04${\scriptstyle\pm0.63}$ & 10.28${\scriptstyle\pm0.75}$ & 9.94${\scriptstyle\pm0.21}$ & 9.99${\scriptstyle\pm0.39}$ & 11.72${\scriptstyle\pm5.07}$ & 15.51${\scriptstyle\pm16.43}$ & 24.11${\scriptstyle\pm28.32}$ & 11.66${\scriptstyle\pm2.94}$ & 16.22${\scriptstyle\pm18.38}$  \\
% GPRGNN & 60.83${\scriptstyle\pm0.75}$ & 59.68${\scriptstyle\pm0.94}$ & 60.47${\scriptstyle\pm1.07}$ & 65.79${\scriptstyle\pm0.7}$ & 75.0${\scriptstyle\pm0.94}$ & 85.79${\scriptstyle\pm1.02}$ & 93.26${\scriptstyle\pm0.78}$ & 97.64${\scriptstyle\pm0.3}$ & 99.38${\scriptstyle\pm0.19}$ & 99.83${\scriptstyle\pm0.08}$ & 99.94${\scriptstyle\pm0.06}$  \\
% FAGCN & 55.89${\scriptstyle\pm0.69}$ & 55.2${\scriptstyle\pm0.59}$ & 56.66${\scriptstyle\pm0.54}$ & 62.08${\scriptstyle\pm0.75}$ & 68.0${\scriptstyle\pm0.78}$ & 76.0${\scriptstyle\pm0.65}$ & 83.38${\scriptstyle\pm0.82}$ & 89.57${\scriptstyle\pm0.53}$ & 93.52${\scriptstyle\pm1.95}$ & 95.93${\scriptstyle\pm1.41}$ & 98.07${\scriptstyle\pm0.48}$  \\
% H2GCN & 62.16${\scriptstyle\pm0.63}$ & 60.77${\scriptstyle\pm0.62}$ & 61.65${\scriptstyle\pm0.71}$ & 66.69${\scriptstyle\pm1.0}$ & 75.48${\scriptstyle\pm1.06}$ & 86.91${\scriptstyle\pm0.6}$ & 93.9${\scriptstyle\pm0.46}$ & 97.76${\scriptstyle\pm0.38}$ & 99.33${\scriptstyle\pm0.14}$ & 99.74${\scriptstyle\pm0.1}$ & 99.92${\scriptstyle\pm0.05}$  \\
% % CPGNN & & & & & & & & & & &  \\
% LP & 9.88${\scriptstyle\pm0.1}$ & 9.96${\scriptstyle\pm0.37}$ & 17.52${\scriptstyle\pm0.44}$ & 27.17${\scriptstyle\pm0.4}$ & 40.96${\scriptstyle\pm0.89}$ & 56.38${\scriptstyle\pm0.87}$ & 74.29${\scriptstyle\pm0.62}$ & 87.39${\scriptstyle\pm0.62}$ & 96.38${\scriptstyle\pm0.17}$ & 99.66${\scriptstyle\pm0.05}$ & 100.0${\scriptstyle\pm0.0}$  \\
% C\&S & 61.97${\scriptstyle\pm0.67}$ & 61.79${\scriptstyle\pm0.83}$ & 62.0${\scriptstyle\pm0.9}$ & 64.82${\scriptstyle\pm0.95}$ & 67.52${\scriptstyle\pm2.9}$ & 72.17${\scriptstyle\pm4.57}$ & 78.18${\scriptstyle\pm6.54}$ & 86.97${\scriptstyle\pm6.39}$ & 96.28${\scriptstyle\pm3.23}$ & 99.49${\scriptstyle\pm0.5}$ & 99.99${\scriptstyle\pm0.03}$  \\
% CLP & 62.59${\scriptstyle\pm0.67}$ & 61.54${\scriptstyle\pm1.1}$ & 62.46${\scriptstyle\pm1.38}$ & 67.29${\scriptstyle\pm1.08}$ & 71.54${\scriptstyle\pm1.12}$ & 77.51${\scriptstyle\pm1.02}$ & 80.94${\scriptstyle\pm1.38}$ & 85.97${\scriptstyle\pm0.92}$ & 90.2${\scriptstyle\pm0.85}$ & 94.63${\scriptstyle\pm0.44}$ & 99.91${\scriptstyle\pm0.06}$  \\
% % \rowcolor{gray!30}
% % CLP\textsuperscript{\dag} & 62.51${\scriptstyle\pm0.78}$ & 62.69${\scriptstyle\pm0.81}$ & 63.8${\scriptstyle\pm0.76}$ & 69.46${\scriptstyle\pm0.55}$ & 74.6${\scriptstyle\pm0.7}$ & 81.11${\scriptstyle\pm0.74}$ & 86.97${\scriptstyle\pm0.49}$ & 91.51${\scriptstyle\pm0.47}$ & 95.55${\scriptstyle\pm0.29}$ & 98.34${\scriptstyle\pm0.09}$ & 99.93${\scriptstyle\pm0.03}$  \\
%         & \multicolumn{11}{c}{\textbf{Train ratio $48\%$}}  \\
% MLP & 71.56${\scriptstyle\pm0.73}$ & 71.36${\scriptstyle\pm1.02}$ & 71.32${\scriptstyle\pm0.82}$ & 72.1${\scriptstyle\pm0.71}$ & 71.54${\scriptstyle\pm0.77}$ & 71.62${\scriptstyle\pm0.72}$ & 71.34${\scriptstyle\pm0.96}$ & 72.09${\scriptstyle\pm0.75}$ & 71.47${\scriptstyle\pm0.85}$ & 71.49${\scriptstyle\pm0.97}$ & 71.54${\scriptstyle\pm0.76}$  \\
% GCN & 31.9${\scriptstyle\pm0.82}$ & 34.86${\scriptstyle\pm1.32}$ & 44.85${\scriptstyle\pm0.92}$ & 58.42${\scriptstyle\pm0.97}$ & 73.85${\scriptstyle\pm0.83}$ & 85.69${\scriptstyle\pm0.61}$ & 93.54${\scriptstyle\pm0.52}$ & 97.37${\scriptstyle\pm0.3}$ & 99.31${\scriptstyle\pm0.16}$ & 99.69${\scriptstyle\pm0.15}$ & 99.89${\scriptstyle\pm0.08}$  \\
% GAT & 9.46${\scriptstyle\pm0.4}$ & 9.33${\scriptstyle\pm0.51}$ & 11.25${\scriptstyle\pm7.9}$ & 9.39${\scriptstyle\pm0.75}$ & 15.44${\scriptstyle\pm17.88}$ & 17.13${\scriptstyle\pm22.87}$ & 9.57${\scriptstyle\pm0.6}$ & 9.82${\scriptstyle\pm0.74}$ & 14.27${\scriptstyle\pm19.48}$ & 12.32${\scriptstyle\pm3.4}$ & 14.28${\scriptstyle\pm19.67}$  \\
% GCN2 & 62.48${\scriptstyle\pm0.71}$ & 62.2${\scriptstyle\pm1.19}$ & 60.5${\scriptstyle\pm0.78}$ & 65.84${\scriptstyle\pm0.89}$ & 71.97${\scriptstyle\pm0.91}$ & 80.25${\scriptstyle\pm0.9}$ & 88.51${\scriptstyle\pm0.42}$ & 94.59${\scriptstyle\pm0.51}$ & 98.56${\scriptstyle\pm0.29}$ & 99.61${\scriptstyle\pm0.15}$ & 99.96${\scriptstyle\pm0.04}$  \\
% SuperGAT & 9.4${\scriptstyle\pm0.49}$ & 9.43${\scriptstyle\pm0.64}$ & 9.43${\scriptstyle\pm0.47}$ & 11.44${\scriptstyle\pm5.81}$ & 10.59${\scriptstyle\pm4.56}$ & 10.06${\scriptstyle\pm1.32}$ & 12.57${\scriptstyle\pm10.57}$ & 21.58${\scriptstyle\pm27.54}$ & 11.88${\scriptstyle\pm9.5}$ & 21.18${\scriptstyle\pm26.31}$ & 13.31${\scriptstyle\pm11.3}$  \\
% GPRGNN & 65.78${\scriptstyle\pm1.03}$ & 63.66${\scriptstyle\pm1.41}$ & 65.0${\scriptstyle\pm1.04}$ & 70.01${\scriptstyle\pm0.67}$ & 76.8${\scriptstyle\pm1.21}$ & 86.15${\scriptstyle\pm1.08}$ & 93.9${\scriptstyle\pm0.57}$ & 97.79${\scriptstyle\pm0.31}$ & 99.54${\scriptstyle\pm0.22}$ & 99.87${\scriptstyle\pm0.07}$ & 99.98${\scriptstyle\pm0.03}$  \\
% FAGCN & 62.03${\scriptstyle\pm1.23}$ & 60.96${\scriptstyle\pm1.12}$ & 62.72${\scriptstyle\pm0.76}$ & 67.94${\scriptstyle\pm0.98}$ & 74.23${\scriptstyle\pm0.75}$ & 82.16${\scriptstyle\pm0.77}$ & 89.3${\scriptstyle\pm0.59}$ & 93.17${\scriptstyle\pm1.53}$ & 96.51${\scriptstyle\pm0.77}$ & 97.9${\scriptstyle\pm0.24}$ & 98.85${\scriptstyle\pm0.28}$  \\
% H2GCN & 75.4${\scriptstyle\pm1.11}$ & 70.31${\scriptstyle\pm1.12}$ & 71.88${\scriptstyle\pm1.0}$ & 79.39${\scriptstyle\pm1.12}$ & 87.56${\scriptstyle\pm0.86}$ & 92.47${\scriptstyle\pm0.61}$ & 96.32${\scriptstyle\pm0.39}$ & 98.49${\scriptstyle\pm0.22}$ & 99.64${\scriptstyle\pm0.13}$ & 99.83${\scriptstyle\pm0.12}$ & 99.98${\scriptstyle\pm0.03}$  \\
% % CPGNN & & & & & & & & & & &  \\
% LP & 9.61${\scriptstyle\pm0.61}$ & 9.56${\scriptstyle\pm0.61}$ & 26.99${\scriptstyle\pm0.79}$ & 47.29${\scriptstyle\pm1.04}$ & 66.89${\scriptstyle\pm1.09}$ & 82.1${\scriptstyle\pm0.83}$ & 92.82${\scriptstyle\pm0.39}$ & 97.86${\scriptstyle\pm0.28}$ & 99.46${\scriptstyle\pm0.16}$ & 99.88${\scriptstyle\pm0.09}$ & 100.0${\scriptstyle\pm0.0}$  \\
% C\&S & 71.36${\scriptstyle\pm0.97}$ & 71.36${\scriptstyle\pm0.91}$ & 72.53${\scriptstyle\pm0.84}$ & 76.13${\scriptstyle\pm1.41}$ & 79.44${\scriptstyle\pm1.88}$ & 84.6${\scriptstyle\pm1.87}$ & 91.27${\scriptstyle\pm1.3}$ & 97.58${\scriptstyle\pm0.55}$ & 99.7${\scriptstyle\pm0.1}$ & 99.96${\scriptstyle\pm0.05}$ & 100.0${\scriptstyle\pm0.01}$  \\
% CLP & 72.55${\scriptstyle\pm1.2}$ & 69.86${\scriptstyle\pm2.41}$ & 72.12${\scriptstyle\pm1.57}$ & 78.15${\scriptstyle\pm1.43}$ & 82.85${\scriptstyle\pm0.9}$ & 86.56${\scriptstyle\pm0.8}$ & 89.79${\scriptstyle\pm0.73}$ & 92.28${\scriptstyle\pm1.09}$ & 94.73${\scriptstyle\pm0.75}$ & 97.14${\scriptstyle\pm0.53}$ & 99.97${\scriptstyle\pm0.04}$  \\
% % \rowcolor{gray!30}
% % CLP\textsuperscript{\dag} & 72.75${\scriptstyle\pm1.04}$ & 72.58${\scriptstyle\pm1.04}$ & 75.08${\scriptstyle\pm0.62}$ & 81.36${\scriptstyle\pm1.04}$ & 86.53${\scriptstyle\pm0.81}$ & 91.0${\scriptstyle\pm0.51}$ & 95.11${\scriptstyle\pm0.53}$ & 97.19${\scriptstyle\pm0.41}$ & 98.75${\scriptstyle\pm0.19}$ & 99.68${\scriptstyle\pm0.12}$ & 99.96${\scriptstyle\pm0.03}$  \\
% \hline
% \end{tabular}
% }
% \end{table*}

% \begin{table*}
% \caption{Node classification results of Syn-Products-3 dataset. 
% % \textsuperscript{\dag} means utilise spectral features.
% }
% % \vspace{-3mm}
% \label{table:NC_experimental_results_p_syn_self_015}
% % \small
% \centering
% \resizebox{.7\textwidth}{!}{
% \begin{tabular}{l ccccccccccc}
% \hline
% $h$     & 0.0 & 0.1 & 0.2 & 0.3 & 0.4 & 0.5 & 0.6 & 0.7 & 0.8 & 0.9 & 1.0\\
%         & \multicolumn{11}{c}{\textbf{Train ratio $5\%$}}  \\
% MLP & 57.47${\scriptstyle\pm0.93}$ & 57.12${\scriptstyle\pm1.13}$ & 57.44${\scriptstyle\pm0.9}$ & 57.58${\scriptstyle\pm1.04}$ & 57.8${\scriptstyle\pm0.75}$ & 56.98${\scriptstyle\pm0.94}$ & 57.94${\scriptstyle\pm1.04}$ & 57.09${\scriptstyle\pm0.73}$ & 57.0${\scriptstyle\pm0.81}$ & 57.72${\scriptstyle\pm1.06}$ & 57.63${\scriptstyle\pm0.83}$  \\
% GCN & 25.5${\scriptstyle\pm0.91}$ & 25.41${\scriptstyle\pm0.5}$ & 34.86${\scriptstyle\pm0.88}$ & 55.35${\scriptstyle\pm0.64}$ & 75.47${\scriptstyle\pm0.85}$ & 90.28${\scriptstyle\pm0.47}$ & 97.12${\scriptstyle\pm0.27}$ & 99.1${\scriptstyle\pm0.21}$ & 99.6${\scriptstyle\pm0.15}$ & 99.77${\scriptstyle\pm0.11}$ & 99.88${\scriptstyle\pm0.12}$  \\
% GAT & 9.91${\scriptstyle\pm0.1}$ & 9.9${\scriptstyle\pm0.17}$ & 10.88${\scriptstyle\pm4.45}$ & 9.92${\scriptstyle\pm0.18}$ & 15.37${\scriptstyle\pm16.68}$ & 14.09${\scriptstyle\pm17.8}$ & 10.15${\scriptstyle\pm0.69}$ & 15.09${\scriptstyle\pm19.37}$ & 12.88${\scriptstyle\pm12.74}$ & 10.43${\scriptstyle\pm2.23}$ & 10.87${\scriptstyle\pm1.46}$  \\
% GCN2 & 50.22${\scriptstyle\pm3.42}$ & 50.01${\scriptstyle\pm1.56}$ & 55.03${\scriptstyle\pm1.67}$ & 61.4${\scriptstyle\pm1.33}$ & 69.85${\scriptstyle\pm1.16}$ & 78.29${\scriptstyle\pm1.07}$ & 88.78${\scriptstyle\pm0.8}$ & 94.58${\scriptstyle\pm0.64}$ & 98.49${\scriptstyle\pm0.26}$ & 99.49${\scriptstyle\pm0.25}$ & 99.8${\scriptstyle\pm0.19}$  \\
% SuperGAT & 9.86${\scriptstyle\pm0.1}$ & 9.93${\scriptstyle\pm0.39}$ & 10.05${\scriptstyle\pm0.68}$ & 9.87${\scriptstyle\pm0.14}$ & 9.94${\scriptstyle\pm0.38}$ & 10.33${\scriptstyle\pm1.02}$ & 15.63${\scriptstyle\pm15.34}$ & 18.21${\scriptstyle\pm21.2}$ & 10.14${\scriptstyle\pm1.1}$ & 14.17${\scriptstyle\pm15.19}$ & 18.68${\scriptstyle\pm24.19}$  \\
% GPRGNN & 57.43${\scriptstyle\pm1.22}$ & 55.91${\scriptstyle\pm1.09}$ & 57.6${\scriptstyle\pm1.52}$ & 66.79${\scriptstyle\pm1.3}$ & 83.44${\scriptstyle\pm0.7}$ & 94.09${\scriptstyle\pm0.55}$ & 98.0${\scriptstyle\pm0.45}$ & 99.21${\scriptstyle\pm0.3}$ & 99.74${\scriptstyle\pm0.12}$ & 99.81${\scriptstyle\pm0.13}$ & 99.89${\scriptstyle\pm0.1}$  \\
% FAGCN & 52.73${\scriptstyle\pm0.98}$ & 51.43${\scriptstyle\pm0.65}$ & 53.1${\scriptstyle\pm1.51}$ & 60.38${\scriptstyle\pm1.21}$ & 67.35${\scriptstyle\pm1.39}$ & 76.6${\scriptstyle\pm0.85}$ & 85.58${\scriptstyle\pm0.96}$ & 90.28${\scriptstyle\pm1.12}$ & 95.05${\scriptstyle\pm0.44}$ & 96.29${\scriptstyle\pm2.55}$ & 97.89${\scriptstyle\pm0.73}$  \\
% H2GCN & 55.53${\scriptstyle\pm0.82}$ & 54.22${\scriptstyle\pm0.93}$ & 55.39${\scriptstyle\pm1.17}$ & 62.68${\scriptstyle\pm1.35}$ & 77.27${\scriptstyle\pm1.91}$ & 91.3${\scriptstyle\pm1.03}$ & 96.83${\scriptstyle\pm0.73}$ & 99.06${\scriptstyle\pm0.34}$ & 99.56${\scriptstyle\pm0.17}$ & 99.83${\scriptstyle\pm0.09}$ & 99.82${\scriptstyle\pm0.2}$  \\
% % CPGNN & & & & & & & & & & &  \\
% LP & 9.9${\scriptstyle\pm0.09}$ & 9.96${\scriptstyle\pm0.22}$ & 16.24${\scriptstyle\pm0.29}$ & 26.01${\scriptstyle\pm0.57}$ & 40.21${\scriptstyle\pm0.86}$ & 58.05${\scriptstyle\pm2.24}$ & 75.48${\scriptstyle\pm1.41}$ & 87.1${\scriptstyle\pm0.58}$ & 96.16${\scriptstyle\pm0.33}$ & 99.78${\scriptstyle\pm0.08}$ & 99.99${\scriptstyle\pm0.01}$  \\
% C\&S & 57.07${\scriptstyle\pm1.01}$ & 56.78${\scriptstyle\pm1.29}$ & 57.39${\scriptstyle\pm1.52}$ & 59.81${\scriptstyle\pm1.88}$ & 64.54${\scriptstyle\pm3.68}$ & 67.57${\scriptstyle\pm6.91}$ & 79.53${\scriptstyle\pm7.75}$ & 86.6${\scriptstyle\pm7.83}$ & 95.16${\scriptstyle\pm6.13}$ & 99.06${\scriptstyle\pm1.72}$ & 100.0${\scriptstyle\pm0.01}$  \\
% CLP & 58.26${\scriptstyle\pm1.35}$ & 56.5${\scriptstyle\pm1.57}$ & 58.59${\scriptstyle\pm1.23}$ & 62.79${\scriptstyle\pm1.37}$ & 67.02${\scriptstyle\pm1.92}$ & 71.53${\scriptstyle\pm1.84}$ & 77.88${\scriptstyle\pm1.79}$ & 83.24${\scriptstyle\pm1.25}$ & 89.02${\scriptstyle\pm1.34}$ & 93.92${\scriptstyle\pm1.17}$ & 99.9${\scriptstyle\pm0.1}$  \\
% % \rowcolor{gray!30}
% % CLP\textsuperscript{\dag} & 57.05${\scriptstyle\pm1.15}$ & 57.27${\scriptstyle\pm0.65}$ & 58.6${\scriptstyle\pm1.35}$ & 63.57${\scriptstyle\pm1.34}$ & 69.67${\scriptstyle\pm1.09}$ & 74.58${\scriptstyle\pm1.08}$ & 81.16${\scriptstyle\pm0.71}$ & 87.39${\scriptstyle\pm0.58}$ & 93.23${\scriptstyle\pm0.61}$ & 97.08${\scriptstyle\pm0.19}$ & 99.85${\scriptstyle\pm0.08}$  \\
%         & \multicolumn{11}{c}{\textbf{Train ratio $10\%$}}  \\
% MLP & 61.83${\scriptstyle\pm0.67}$ & 61.69${\scriptstyle\pm0.87}$ & 61.99${\scriptstyle\pm0.86}$ & 61.91${\scriptstyle\pm0.75}$ & 62.41${\scriptstyle\pm0.68}$ & 61.89${\scriptstyle\pm0.69}$ & 62.24${\scriptstyle\pm0.66}$ & 61.53${\scriptstyle\pm0.79}$ & 61.84${\scriptstyle\pm0.69}$ & 61.6${\scriptstyle\pm0.54}$ & 61.77${\scriptstyle\pm0.61}$  \\
% GCN & 27.85${\scriptstyle\pm0.62}$ & 28.52${\scriptstyle\pm0.55}$ & 38.77${\scriptstyle\pm0.59}$ & 59.21${\scriptstyle\pm0.43}$ & 78.97${\scriptstyle\pm0.41}$ & 91.64${\scriptstyle\pm0.36}$ & 97.46${\scriptstyle\pm0.18}$ & 99.22${\scriptstyle\pm0.11}$ & 99.75${\scriptstyle\pm0.08}$ & 99.93${\scriptstyle\pm0.05}$ & 99.92${\scriptstyle\pm0.06}$  \\
% GAT & 9.81${\scriptstyle\pm0.1}$ & 9.93${\scriptstyle\pm0.36}$ & 9.87${\scriptstyle\pm0.15}$ & 12.44${\scriptstyle\pm11.11}$ & 10.93${\scriptstyle\pm4.46}$ & 10.07${\scriptstyle\pm0.53}$ & 10.24${\scriptstyle\pm1.01}$ & 10.97${\scriptstyle\pm2.03}$ & 23.34${\scriptstyle\pm31.99}$ & 10.35${\scriptstyle\pm1.2}$ & 11.87${\scriptstyle\pm3.18}$  \\
% GCN2 & 57.32${\scriptstyle\pm1.0}$ & 55.26${\scriptstyle\pm2.23}$ & 57.25${\scriptstyle\pm1.76}$ & 63.94${\scriptstyle\pm0.78}$ & 72.68${\scriptstyle\pm0.66}$ & 81.29${\scriptstyle\pm1.18}$ & 89.82${\scriptstyle\pm0.59}$ & 95.43${\scriptstyle\pm0.31}$ & 98.72${\scriptstyle\pm0.25}$ & 99.71${\scriptstyle\pm0.09}$ & 99.95${\scriptstyle\pm0.05}$  \\
% SuperGAT & 9.84${\scriptstyle\pm0.22}$ & 9.92${\scriptstyle\pm0.18}$ & 9.9${\scriptstyle\pm0.14}$ & 10.75${\scriptstyle\pm4.05}$ & 11.23${\scriptstyle\pm5.78}$ & 10.02${\scriptstyle\pm0.51}$ & 16.22${\scriptstyle\pm17.57}$ & 11.39${\scriptstyle\pm2.0}$ & 9.86${\scriptstyle\pm0.18}$ & 15.74${\scriptstyle\pm16.39}$ & 19.38${\scriptstyle\pm26.8}$  \\
% GPRGNN & 61.82${\scriptstyle\pm0.61}$ & 58.88${\scriptstyle\pm1.26}$ & 61.35${\scriptstyle\pm0.81}$ & 69.86${\scriptstyle\pm0.73}$ & 85.01${\scriptstyle\pm0.86}$ & 94.64${\scriptstyle\pm0.58}$ & 98.17${\scriptstyle\pm0.32}$ & 99.46${\scriptstyle\pm0.15}$ & 99.85${\scriptstyle\pm0.08}$ & 99.91${\scriptstyle\pm0.06}$ & 99.94${\scriptstyle\pm0.07}$  \\
% FAGCN & 55.85${\scriptstyle\pm0.72}$ & 54.99${\scriptstyle\pm0.63}$ & 57.41${\scriptstyle\pm0.77}$ & 64.13${\scriptstyle\pm0.79}$ & 72.63${\scriptstyle\pm0.9}$ & 80.94${\scriptstyle\pm0.9}$ & 87.62${\scriptstyle\pm2.84}$ & 92.57${\scriptstyle\pm0.5}$ & 95.85${\scriptstyle\pm1.41}$ & 98.13${\scriptstyle\pm0.2}$ & 98.35${\scriptstyle\pm0.63}$  \\
% H2GCN & 62.31${\scriptstyle\pm0.79}$ & 60.73${\scriptstyle\pm0.83}$ & 61.94${\scriptstyle\pm1.04}$ & 69.94${\scriptstyle\pm0.79}$ & 83.86${\scriptstyle\pm1.4}$ & 93.36${\scriptstyle\pm0.93}$ & 97.57${\scriptstyle\pm0.32}$ & 99.27${\scriptstyle\pm0.23}$ & 99.76${\scriptstyle\pm0.12}$ & 99.86${\scriptstyle\pm0.08}$ & 99.94${\scriptstyle\pm0.07}$  \\
% % CPGNN & & & & & & & & & & &  \\
% LP & 9.81${\scriptstyle\pm0.1}$ & 10.1${\scriptstyle\pm0.22}$ & 19.4${\scriptstyle\pm0.22}$ & 31.76${\scriptstyle\pm0.43}$ & 48.44${\scriptstyle\pm0.45}$ & 65.5${\scriptstyle\pm0.74}$ & 81.29${\scriptstyle\pm0.75}$ & 92.91${\scriptstyle\pm0.35}$ & 99.16${\scriptstyle\pm0.11}$ & 99.95${\scriptstyle\pm0.04}$ & 100.0${\scriptstyle\pm0.01}$  \\
% C\&S & 61.7${\scriptstyle\pm0.75}$ & 61.33${\scriptstyle\pm0.8}$ & 62.65${\scriptstyle\pm0.97}$ & 64.77${\scriptstyle\pm1.28}$ & 69.78${\scriptstyle\pm4.15}$ & 71.37${\scriptstyle\pm6.4}$ & 79.02${\scriptstyle\pm8.49}$ & 87.88${\scriptstyle\pm7.23}$ & 95.58${\scriptstyle\pm3.27}$ & 99.87${\scriptstyle\pm0.15}$ & 99.99${\scriptstyle\pm0.02}$  \\
% CLP & 63.25${\scriptstyle\pm1.6}$ & 61.14${\scriptstyle\pm1.27}$ & 63.74${\scriptstyle\pm0.94}$ & 68.1${\scriptstyle\pm1.03}$ & 73.92${\scriptstyle\pm1.2}$ & 78.24${\scriptstyle\pm1.01}$ & 83.12${\scriptstyle\pm1.06}$ & 86.51${\scriptstyle\pm1.24}$ & 89.34${\scriptstyle\pm0.85}$ & 94.6${\scriptstyle\pm0.81}$ & 99.9${\scriptstyle\pm0.09}$  \\
% % \rowcolor{gray!30}
% % CLP\textsuperscript{\dag} & 62.11${\scriptstyle\pm0.55}$ & 62.03${\scriptstyle\pm0.79}$ & 64.68${\scriptstyle\pm0.88}$ & 70.12${\scriptstyle\pm0.61}$ & 76.34${\scriptstyle\pm0.68}$ & 82.31${\scriptstyle\pm0.67}$ & 87.9${\scriptstyle\pm0.48}$ & 92.04${\scriptstyle\pm0.43}$ & 95.7${\scriptstyle\pm0.34}$ & 98.44${\scriptstyle\pm0.18}$ & 99.92${\scriptstyle\pm0.03}$  \\
%         & \multicolumn{11}{c}{\textbf{Train ratio $48\%$}}  \\
% MLP & 71.74${\scriptstyle\pm0.95}$ & 71.96${\scriptstyle\pm0.95}$ & 72.17${\scriptstyle\pm1.0}$ & 72.15${\scriptstyle\pm0.87}$ & 72.43${\scriptstyle\pm0.76}$ & 71.52${\scriptstyle\pm0.84}$ & 71.87${\scriptstyle\pm0.78}$ & 71.25${\scriptstyle\pm1.21}$ & 70.82${\scriptstyle\pm1.1}$ & 72.25${\scriptstyle\pm0.73}$ & 71.68${\scriptstyle\pm1.05}$  \\
% GCN & 33.97${\scriptstyle\pm0.94}$ & 34.45${\scriptstyle\pm1.03}$ & 45.69${\scriptstyle\pm1.12}$ & 65.76${\scriptstyle\pm0.7}$ & 83.11${\scriptstyle\pm0.91}$ & 93.78${\scriptstyle\pm0.54}$ & 97.92${\scriptstyle\pm0.35}$ & 99.48${\scriptstyle\pm0.16}$ & 99.85${\scriptstyle\pm0.1}$ & 99.95${\scriptstyle\pm0.05}$ & 100.0${\scriptstyle\pm0.01}$  \\
% GAT & 9.26${\scriptstyle\pm0.39}$ & 9.61${\scriptstyle\pm0.81}$ & 9.69${\scriptstyle\pm0.63}$ & 9.57${\scriptstyle\pm0.63}$ & 9.2${\scriptstyle\pm0.53}$ & 10.25${\scriptstyle\pm1.12}$ & 10.0${\scriptstyle\pm1.46}$ & 9.8${\scriptstyle\pm1.26}$ & 17.1${\scriptstyle\pm21.11}$ & 10.67${\scriptstyle\pm1.87}$ & 11.18${\scriptstyle\pm3.48}$  \\
% GCN2 & 62.8${\scriptstyle\pm0.83}$ & 62.85${\scriptstyle\pm1.3}$ & 62.09${\scriptstyle\pm1.13}$ & 67.53${\scriptstyle\pm0.96}$ & 75.74${\scriptstyle\pm0.82}$ & 83.85${\scriptstyle\pm0.64}$ & 91.52${\scriptstyle\pm0.79}$ & 96.23${\scriptstyle\pm0.31}$ & 98.98${\scriptstyle\pm0.16}$ & 99.8${\scriptstyle\pm0.09}$ & 99.97${\scriptstyle\pm0.04}$  \\
% SuperGAT & 9.31${\scriptstyle\pm0.43}$ & 9.73${\scriptstyle\pm2.37}$ & 9.62${\scriptstyle\pm0.43}$ & 9.54${\scriptstyle\pm0.41}$ & 9.53${\scriptstyle\pm0.6}$ & 10.04${\scriptstyle\pm1.07}$ & 10.23${\scriptstyle\pm1.16}$ & 22.94${\scriptstyle\pm29.69}$ & 12.07${\scriptstyle\pm5.55}$ & 26.94${\scriptstyle\pm34.23}$ & 19.62${\scriptstyle\pm23.77}$  \\
% GPRGNN & 66.59${\scriptstyle\pm1.21}$ & 64.26${\scriptstyle\pm1.06}$ & 66.54${\scriptstyle\pm0.99}$ & 73.5${\scriptstyle\pm1.07}$ & 85.86${\scriptstyle\pm0.95}$ & 95.16${\scriptstyle\pm0.59}$ & 98.28${\scriptstyle\pm0.32}$ & 99.42${\scriptstyle\pm0.24}$ & 99.91${\scriptstyle\pm0.06}$ & 99.98${\scriptstyle\pm0.03}$ & 99.97${\scriptstyle\pm0.04}$  \\
% FAGCN & 62.81${\scriptstyle\pm1.03}$ & 61.92${\scriptstyle\pm1.34}$ & 63.22${\scriptstyle\pm1.05}$ & 70.47${\scriptstyle\pm1.03}$ & 79.81${\scriptstyle\pm0.82}$ & 88.09${\scriptstyle\pm1.15}$ & 94.06${\scriptstyle\pm0.92}$ & 96.69${\scriptstyle\pm0.86}$ & 97.82${\scriptstyle\pm0.36}$ & 98.88${\scriptstyle\pm0.22}$ & 99.26${\scriptstyle\pm0.16}$  \\
% H2GCN & 78.58${\scriptstyle\pm1.04}$ & 70.9${\scriptstyle\pm0.76}$ & 72.94${\scriptstyle\pm1.1}$ & 83.25${\scriptstyle\pm1.18}$ & 91.24${\scriptstyle\pm0.94}$ & 96.13${\scriptstyle\pm0.49}$ & 98.82${\scriptstyle\pm0.22}$ & 99.64${\scriptstyle\pm0.15}$ & 99.91${\scriptstyle\pm0.06}$ & 99.95${\scriptstyle\pm0.04}$ & 99.98${\scriptstyle\pm0.03}$  \\
% % CPGNN & & & & & & & & & & &  \\
% LP & 9.54${\scriptstyle\pm0.63}$ & 9.57${\scriptstyle\pm0.75}$ & 31.15${\scriptstyle\pm0.42}$ & 56.28${\scriptstyle\pm1.2}$ & 78.28${\scriptstyle\pm1.07}$ & 91.86${\scriptstyle\pm0.57}$ & 97.9${\scriptstyle\pm0.34}$ & 99.5${\scriptstyle\pm0.2}$ & 99.91${\scriptstyle\pm0.05}$ & 99.97${\scriptstyle\pm0.04}$ & 100.0${\scriptstyle\pm0.0}$  \\
% C\&S & 71.63${\scriptstyle\pm1.04}$ & 71.78${\scriptstyle\pm0.74}$ & 73.94${\scriptstyle\pm0.96}$ & 75.99${\scriptstyle\pm1.18}$ & 79.96${\scriptstyle\pm1.75}$ & 84.48${\scriptstyle\pm2.09}$ & 92.09${\scriptstyle\pm1.99}$ & 97.86${\scriptstyle\pm0.7}$ & 99.89${\scriptstyle\pm0.08}$ & 100.0${\scriptstyle\pm0.01}$ & 99.99${\scriptstyle\pm0.04}$  \\
% CLP & 73.93${\scriptstyle\pm2.12}$ & 70.73${\scriptstyle\pm2.31}$ & 74.44${\scriptstyle\pm1.93}$ & 80.22${\scriptstyle\pm0.94}$ & 84.78${\scriptstyle\pm0.97}$ & 88.68${\scriptstyle\pm0.82}$ & 91.36${\scriptstyle\pm1.13}$ & 92.95${\scriptstyle\pm1.12}$ & 95.05${\scriptstyle\pm1.03}$ & 97.54${\scriptstyle\pm0.53}$ & 99.98${\scriptstyle\pm0.04}$  \\
% % \rowcolor{gray!30}
% % CLP\textsuperscript{\dag} & 72.34${\scriptstyle\pm0.92}$ & 72.54${\scriptstyle\pm0.75}$ & 76.74${\scriptstyle\pm0.94}$ & 82.81${\scriptstyle\pm0.66}$ & 89.23${\scriptstyle\pm0.6}$ & 93.53${\scriptstyle\pm0.5}$ & 96.22${\scriptstyle\pm0.31}$ & 97.63${\scriptstyle\pm0.33}$ & 99.08${\scriptstyle\pm0.21}$ & 99.78${\scriptstyle\pm0.1}$ & 100.0${\scriptstyle\pm0.01}$  \\
% \hline
% \end{tabular}
% }
% \end{table*}

% As supplemental results of Figure~\ref{fig:accuracy_diff_methods_diff_syn_data} in Section~\ref{subsec:experimental_results_syn},
% Table~\ref{table:NC_experimental_results_syn_self_005}, Table~\ref{table:NC_experimental_results_syn_self_010} and Table~\ref{table:NC_experimental_results_syn_self_015} give the detailed node classification performance on three synthetic datasets with statistic node features with \textit{sparse}, \textit{medium} and \textit{dense} splittings. 
% Table~\ref{table:NC_experimental_results_p_syn_self_005}, Table~\ref{table:NC_experimental_results_p_syn_self_010} and Table~\ref{table:NC_experimental_results_p_syn_self_015} give the detailed node classification performance on three synthetic datasets with real-world node features with \textit{sparse}, \textit{medium} and \textit{dense} splittings. 
